# Supplementary material for: InfoLM: A New Metric to Evaluate Summarization & Data2Text Generation
Source: arXiv:2112.01589 source file (2022-03-25)
Supplement: Supplementary file 1 [file appendix.tex]

\section{Additional Experimental Results}
In this section, we report the additional experiments we conduct. Because of space constraints, we did not report the sensibility analysis (see \cref{ssec:choice_of_alpha_beta}) in the main paper. 
\subsection{Role of calibration}\label{ssec:role_of_calibration_additional_details}
The complete results on the role of calibration can be found in \cref{fig:calibration_rao_all_total}. We notice a similar behaviour for \texttt{InfoLM} on both extractive and abstractive systems. There is a smooth variation in terms of performance and a single maximum for $\mathcal{T} \in [1,2]$. 

\begin{figure*}[!htb]
           \centering
    \subfloat[Abstractive]{{\includegraphics[width=0.5\textwidth]{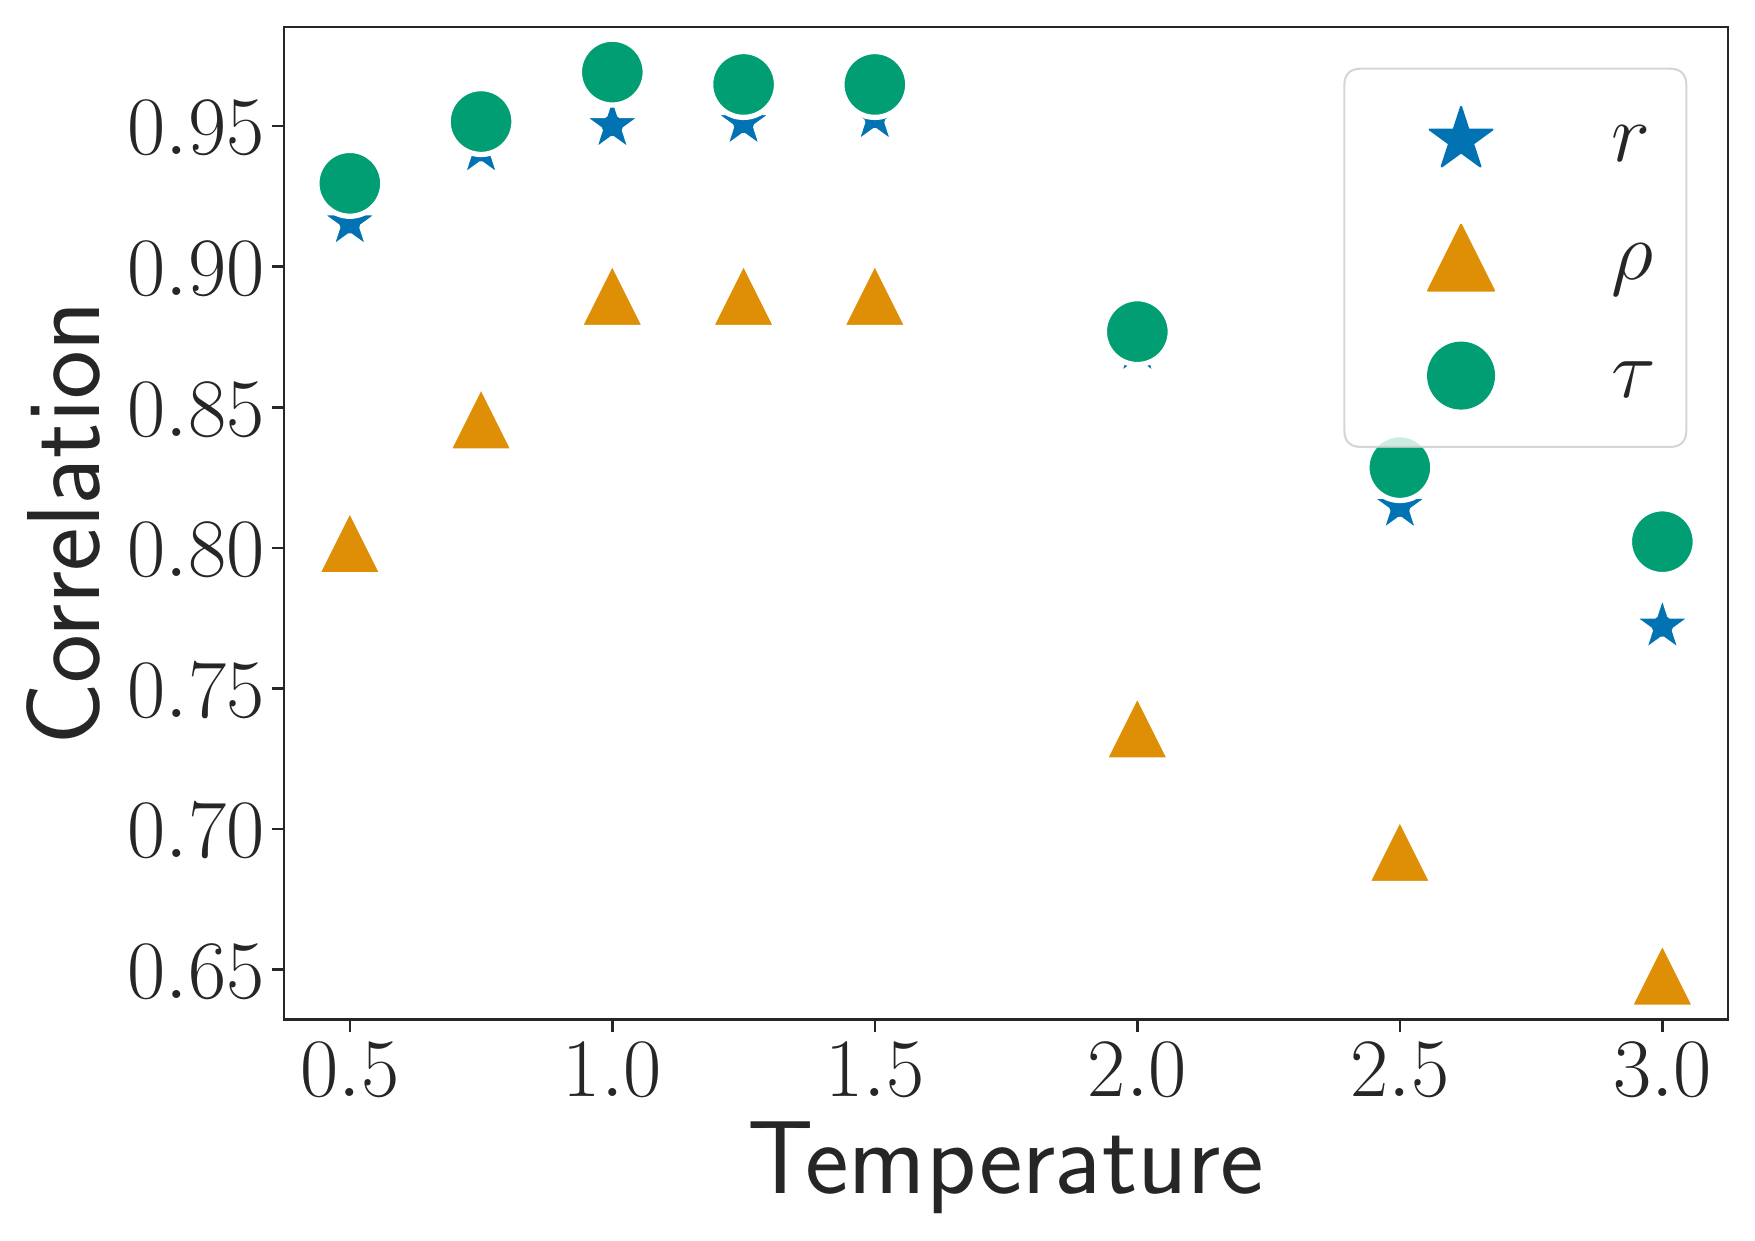} }}
    %\qquad
    \subfloat[Extractive]{{\includegraphics[width=0.5\textwidth]{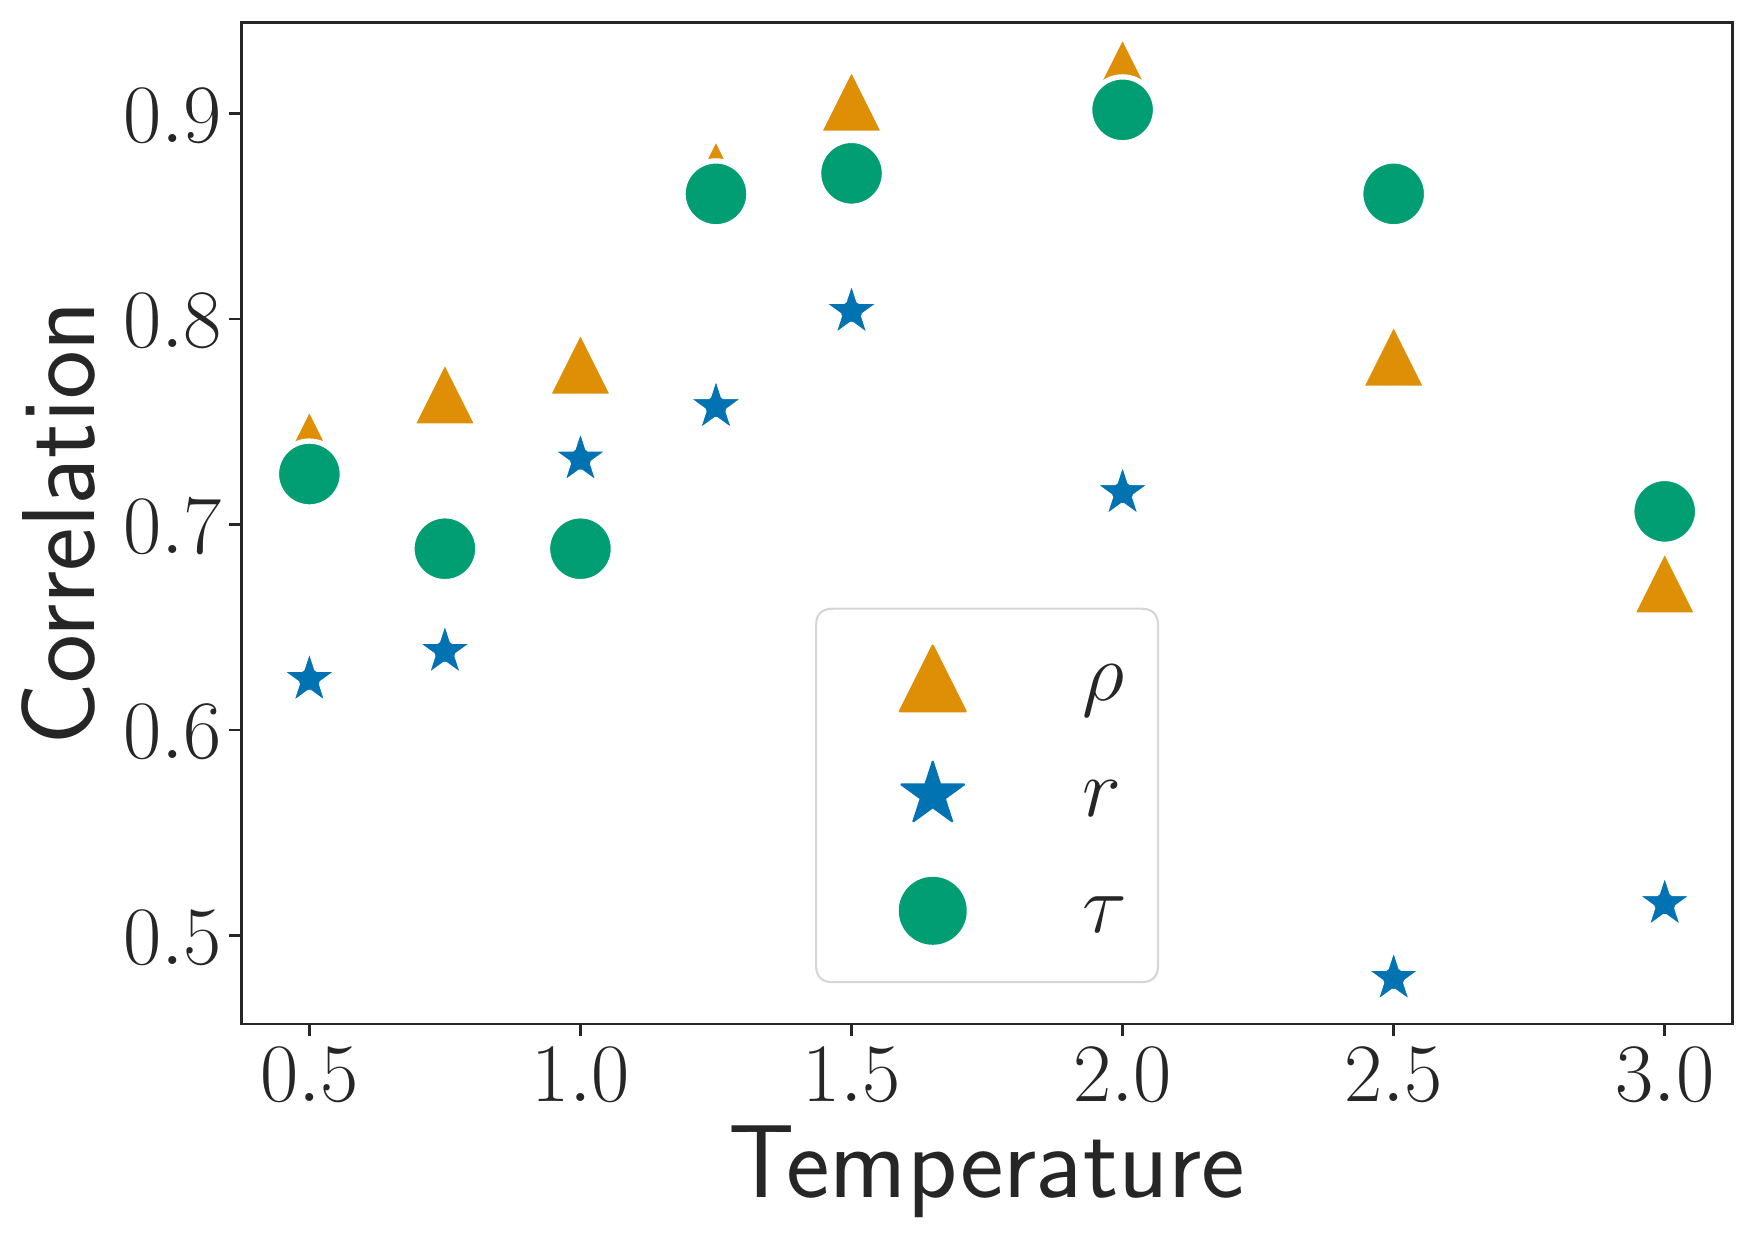} }}
    \caption{Impact of Calibration on system-level correlation (with Pearson ($r$), Spearman ($\rho$) or Kendall ($\tau$)) for CNN. The chosen measure is Rao as it is parameter-free. Calibration is changed using temperature scaling using a single temperature $\mathcal{T}$.}\label{fig:calibration_rao_all_total}
\end{figure*}

\subsection{Choice of $\alpha$ and $\beta$}\label{ssec:choice_of_alpha_beta}
In this experiment, we aim at quantifying the sensitivity of $\mathcal{D}_{AB}$ to the choice of $\alpha$ and $\beta$. \cref{fig:sensibility} gathers the results of the analysis. We observe that a change in $\beta$ induces a stronger change in the metric. Additionally the lower $\beta$ the better result we obtain. We can also note that the variation of both parameters is smooth. Interestingly for abstractive systems, a low value of $\alpha$ should be chosen where for extractive higher is better. It suggests that for evaluating abstractive systems the metric should focus on low values of $p_i/q_i$ (words that are probable for both candidate and reference text) where for extractive systems the attention should be focused on high values of $p_i/q_i$ (words that are likely only in one text).
\\\textbf{Takeaways.} Low values of $\beta$ leads to better results, optimal value of $\alpha$ is $1.25$ for abstractive and $3$ for extractive. Good parameter combinations achieve consistently high performance when using different correlation coefficients.
\begin{figure*}[htp]
\centering
 \includegraphics[width=.4\textwidth]{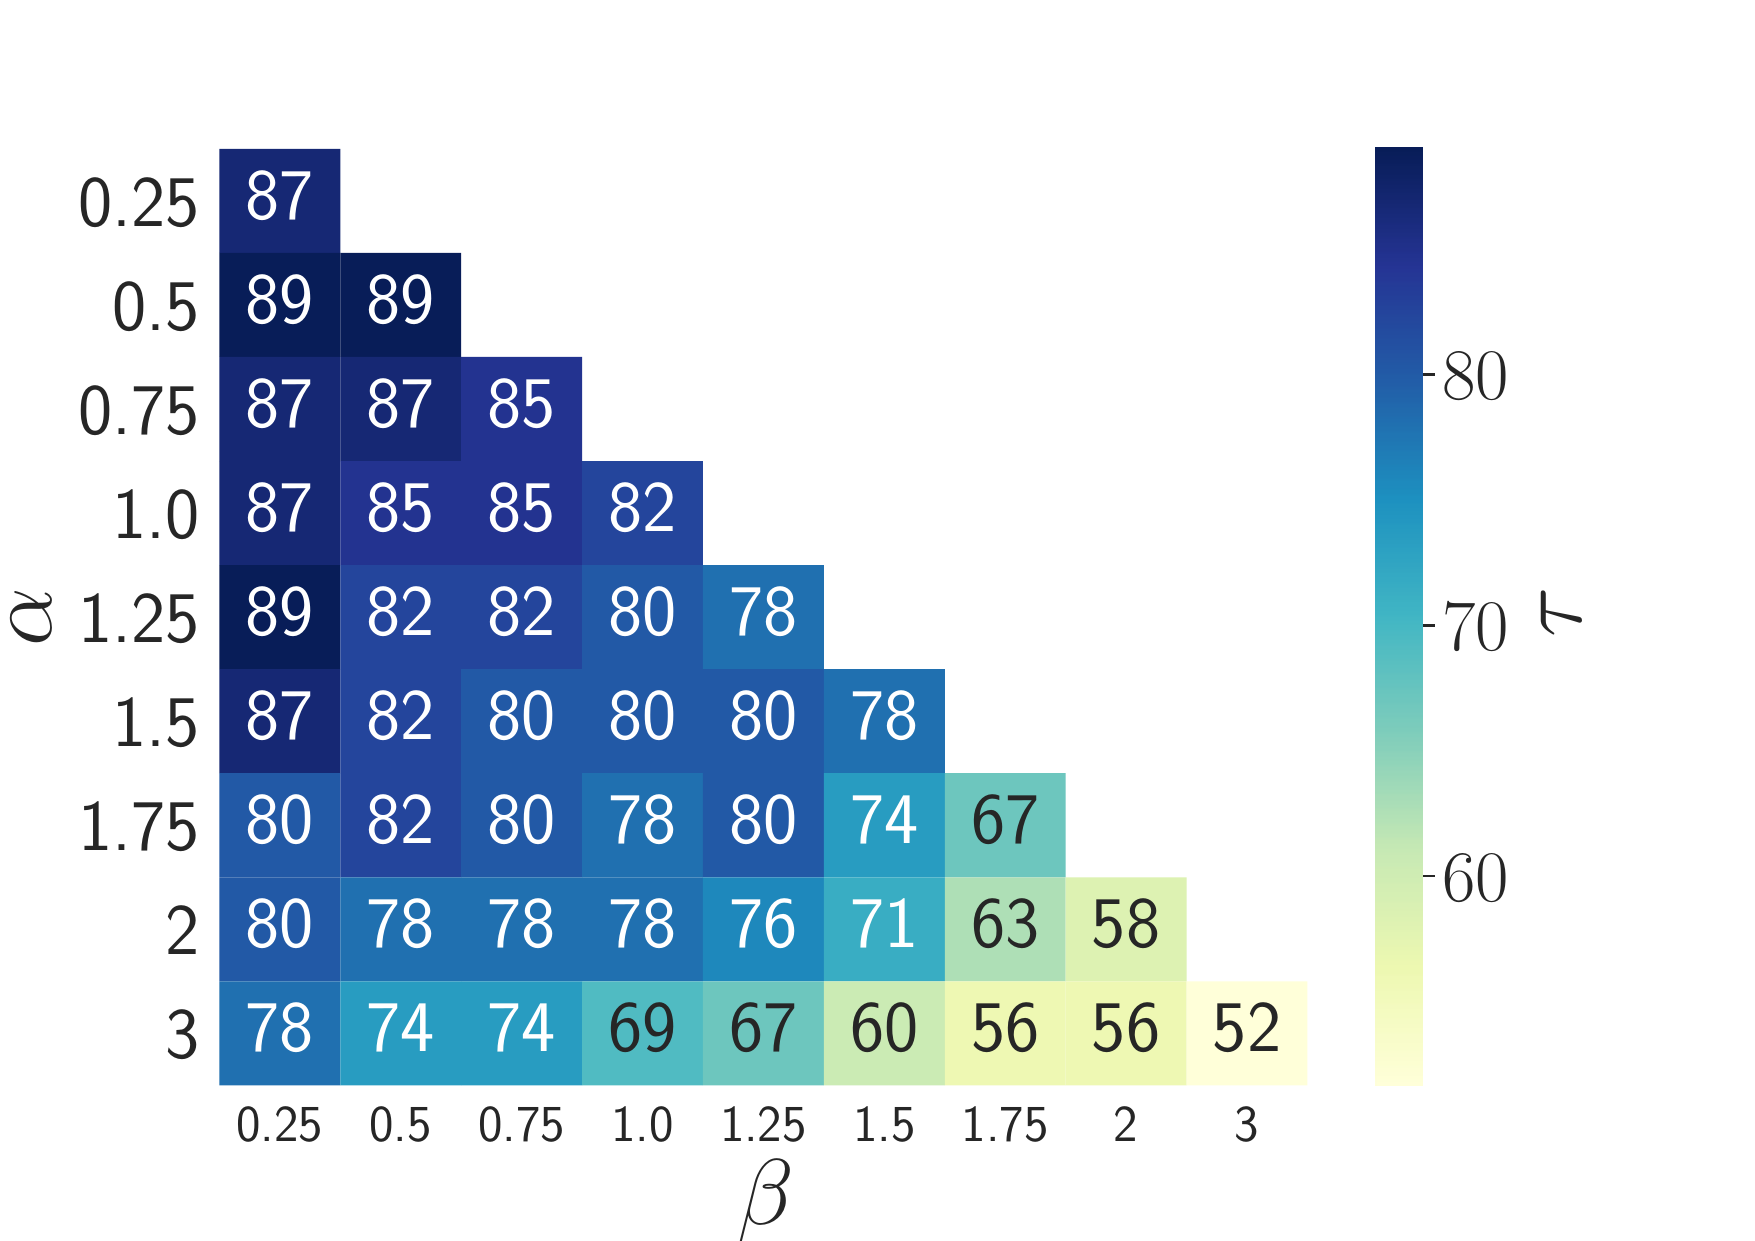}
\includegraphics[width=.4\textwidth]{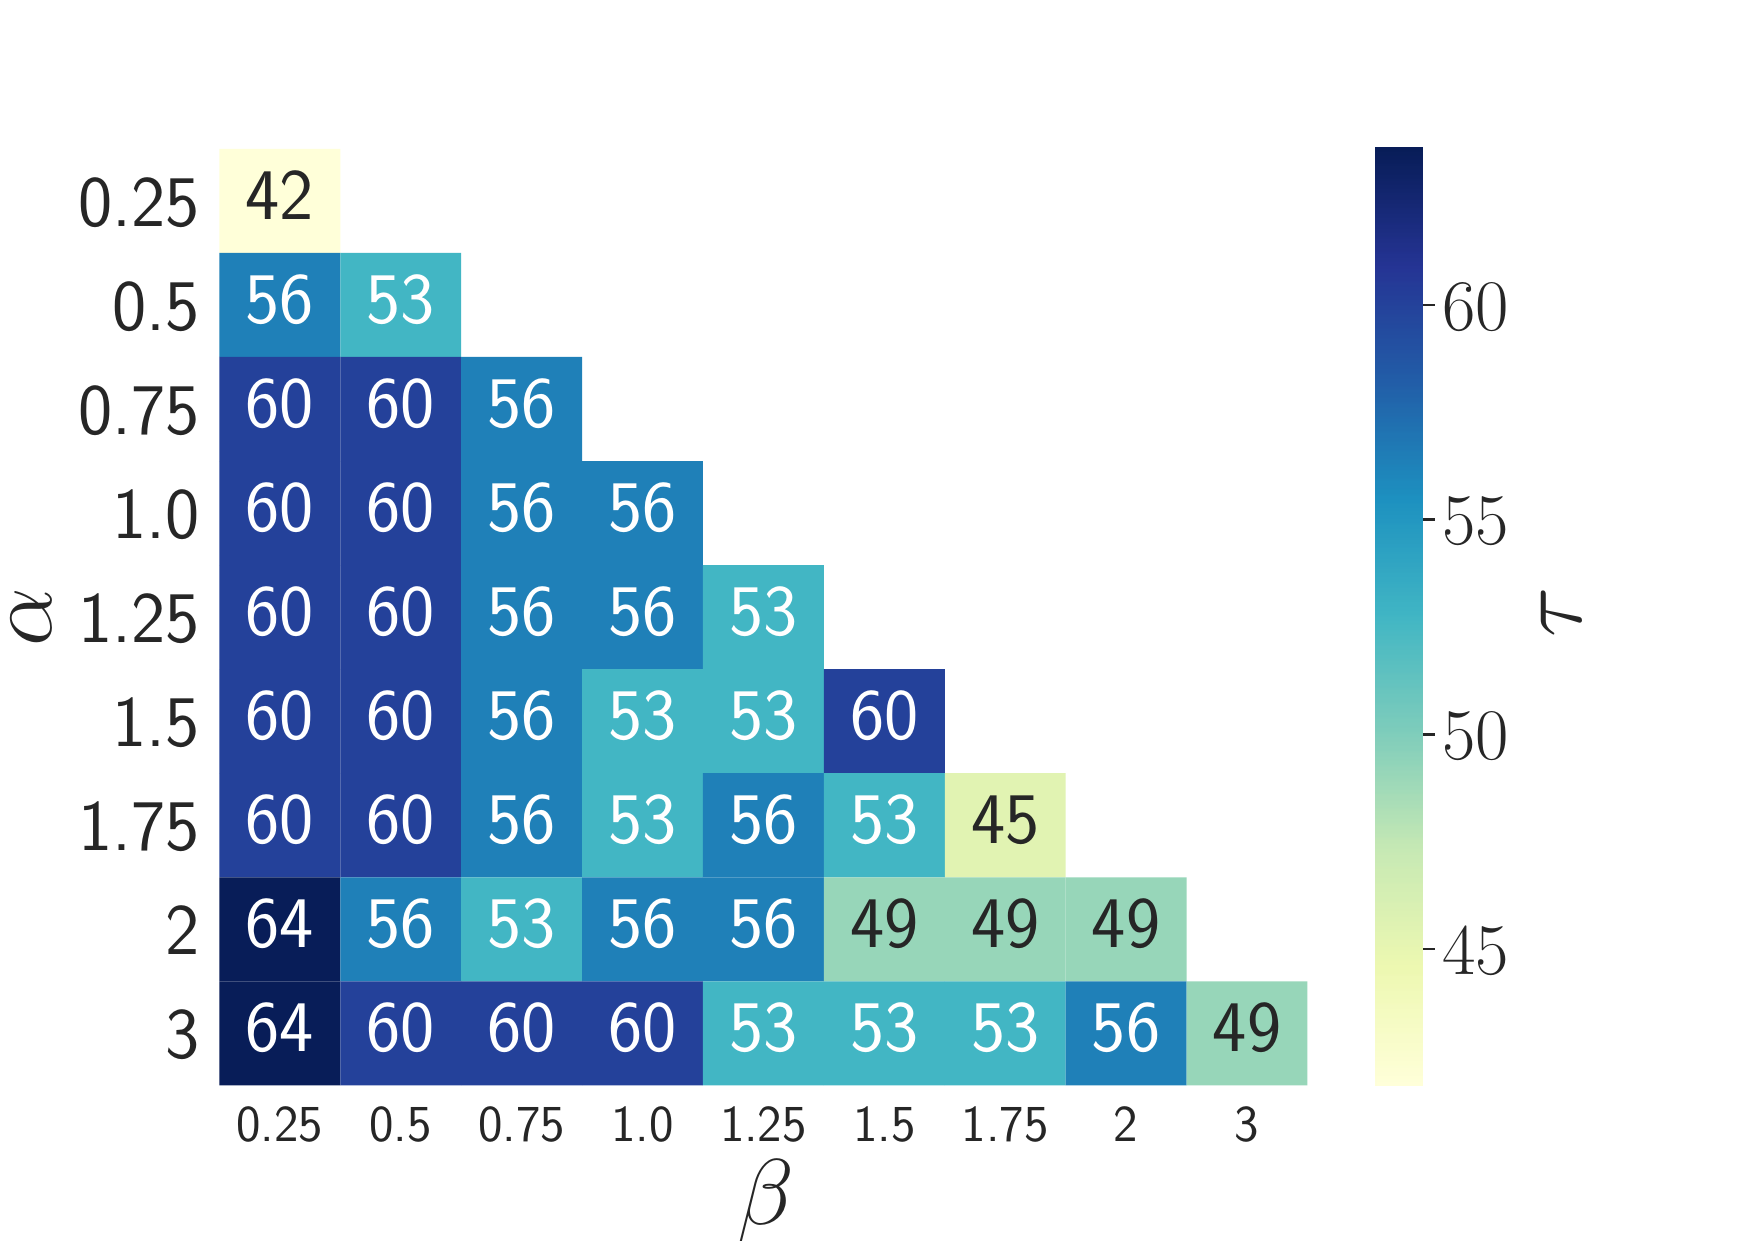} \\
\includegraphics[width=.4\textwidth]{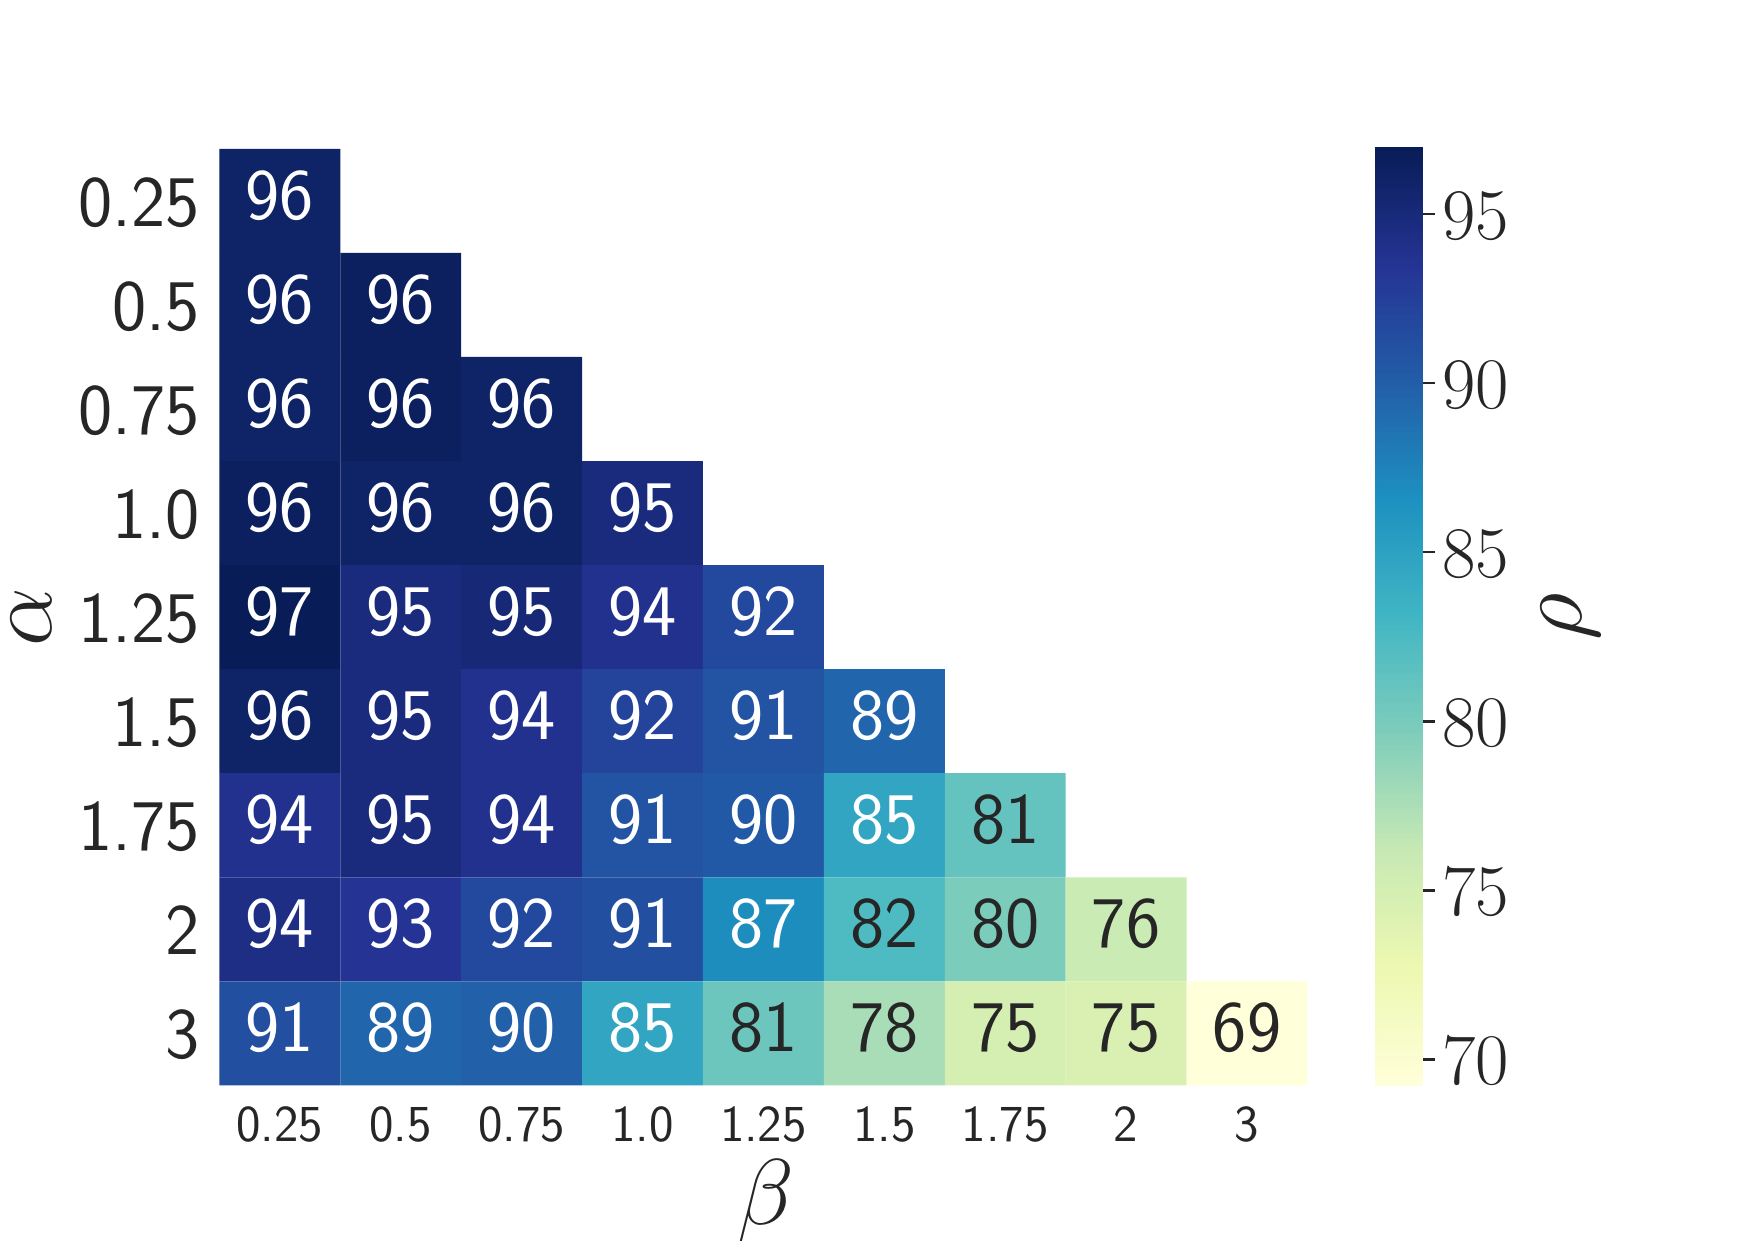}
\includegraphics[width=.4\textwidth]{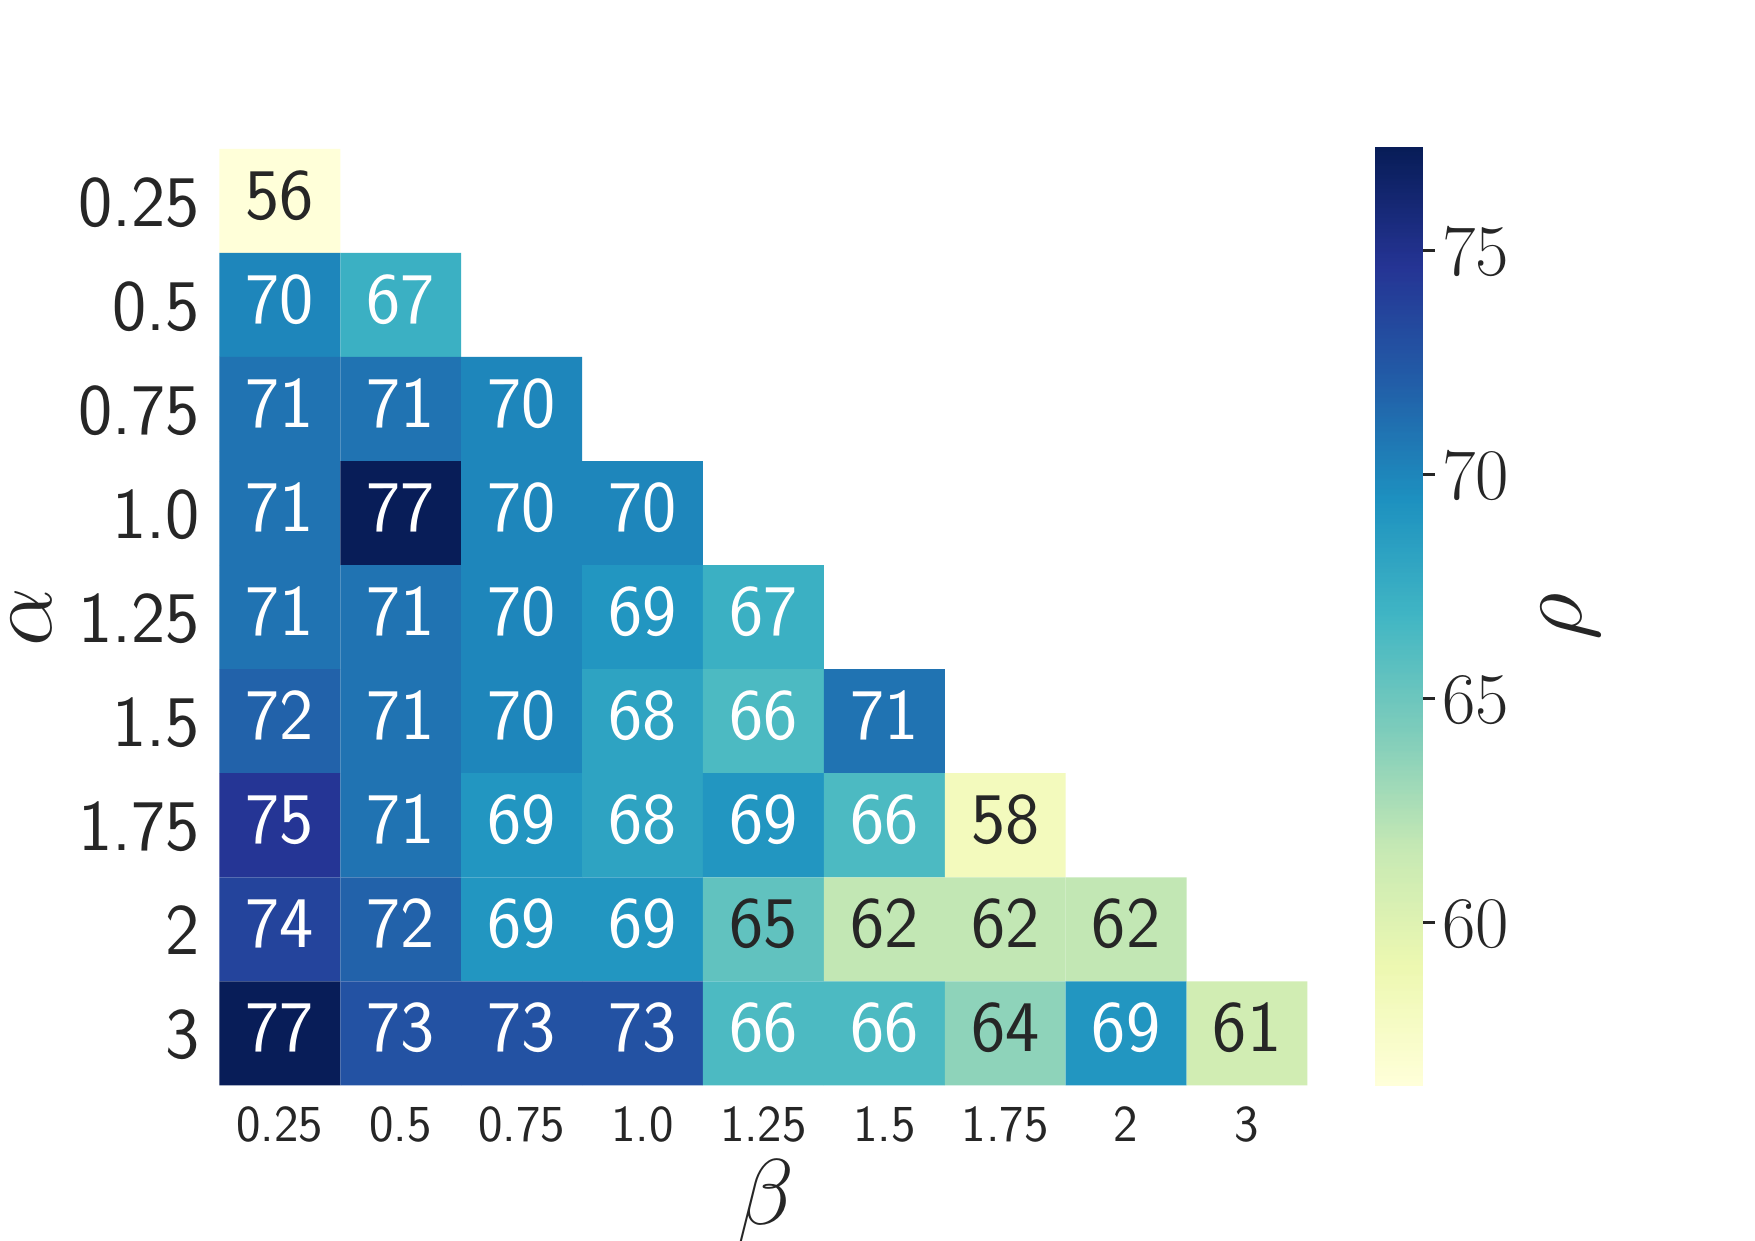}
\caption{Impact of change in $\alpha$ and $\beta$ for $\mathcal{D}_{AB}$ . System level correlation, as measured by Pearson ($r$) or Spearman ($\rho$), is presented on abstractive (first column) and extractive system (second column).}\label{fig:sensibility}
\end{figure*}

\subsection{Statistical analysis}\label{ssec:statistical_analysis}
Automatic metrics are used in the WebNLG challenge to compare the different systems. To evaluate whether the observed improvement in correlation is significant, we report the results of William's Significance test in \cref{fig:william}. 
\\\textbf{Takeaways:} (i) Regarding correctness and relevance $\mathcal{D}_{AB}$, is a suitable choice that is significantly better than other metrics; (ii) Regarding text structure, $\mathcal{R}$ is significantly better and compare favourably against all metrics except \texttt{MOVERSCORE} for automatic fluency evaluation; (iii) Regarding data coverage, \texttt{METEOR} achieves good result however significance difference is only observed with \texttt{BERTSCORE}.
\begin{figure*}[!htb]
   \begin{minipage}{0.22\textwidth}
     \centering
      \subfloat[Correct]{ \includegraphics[width=\linewidth]{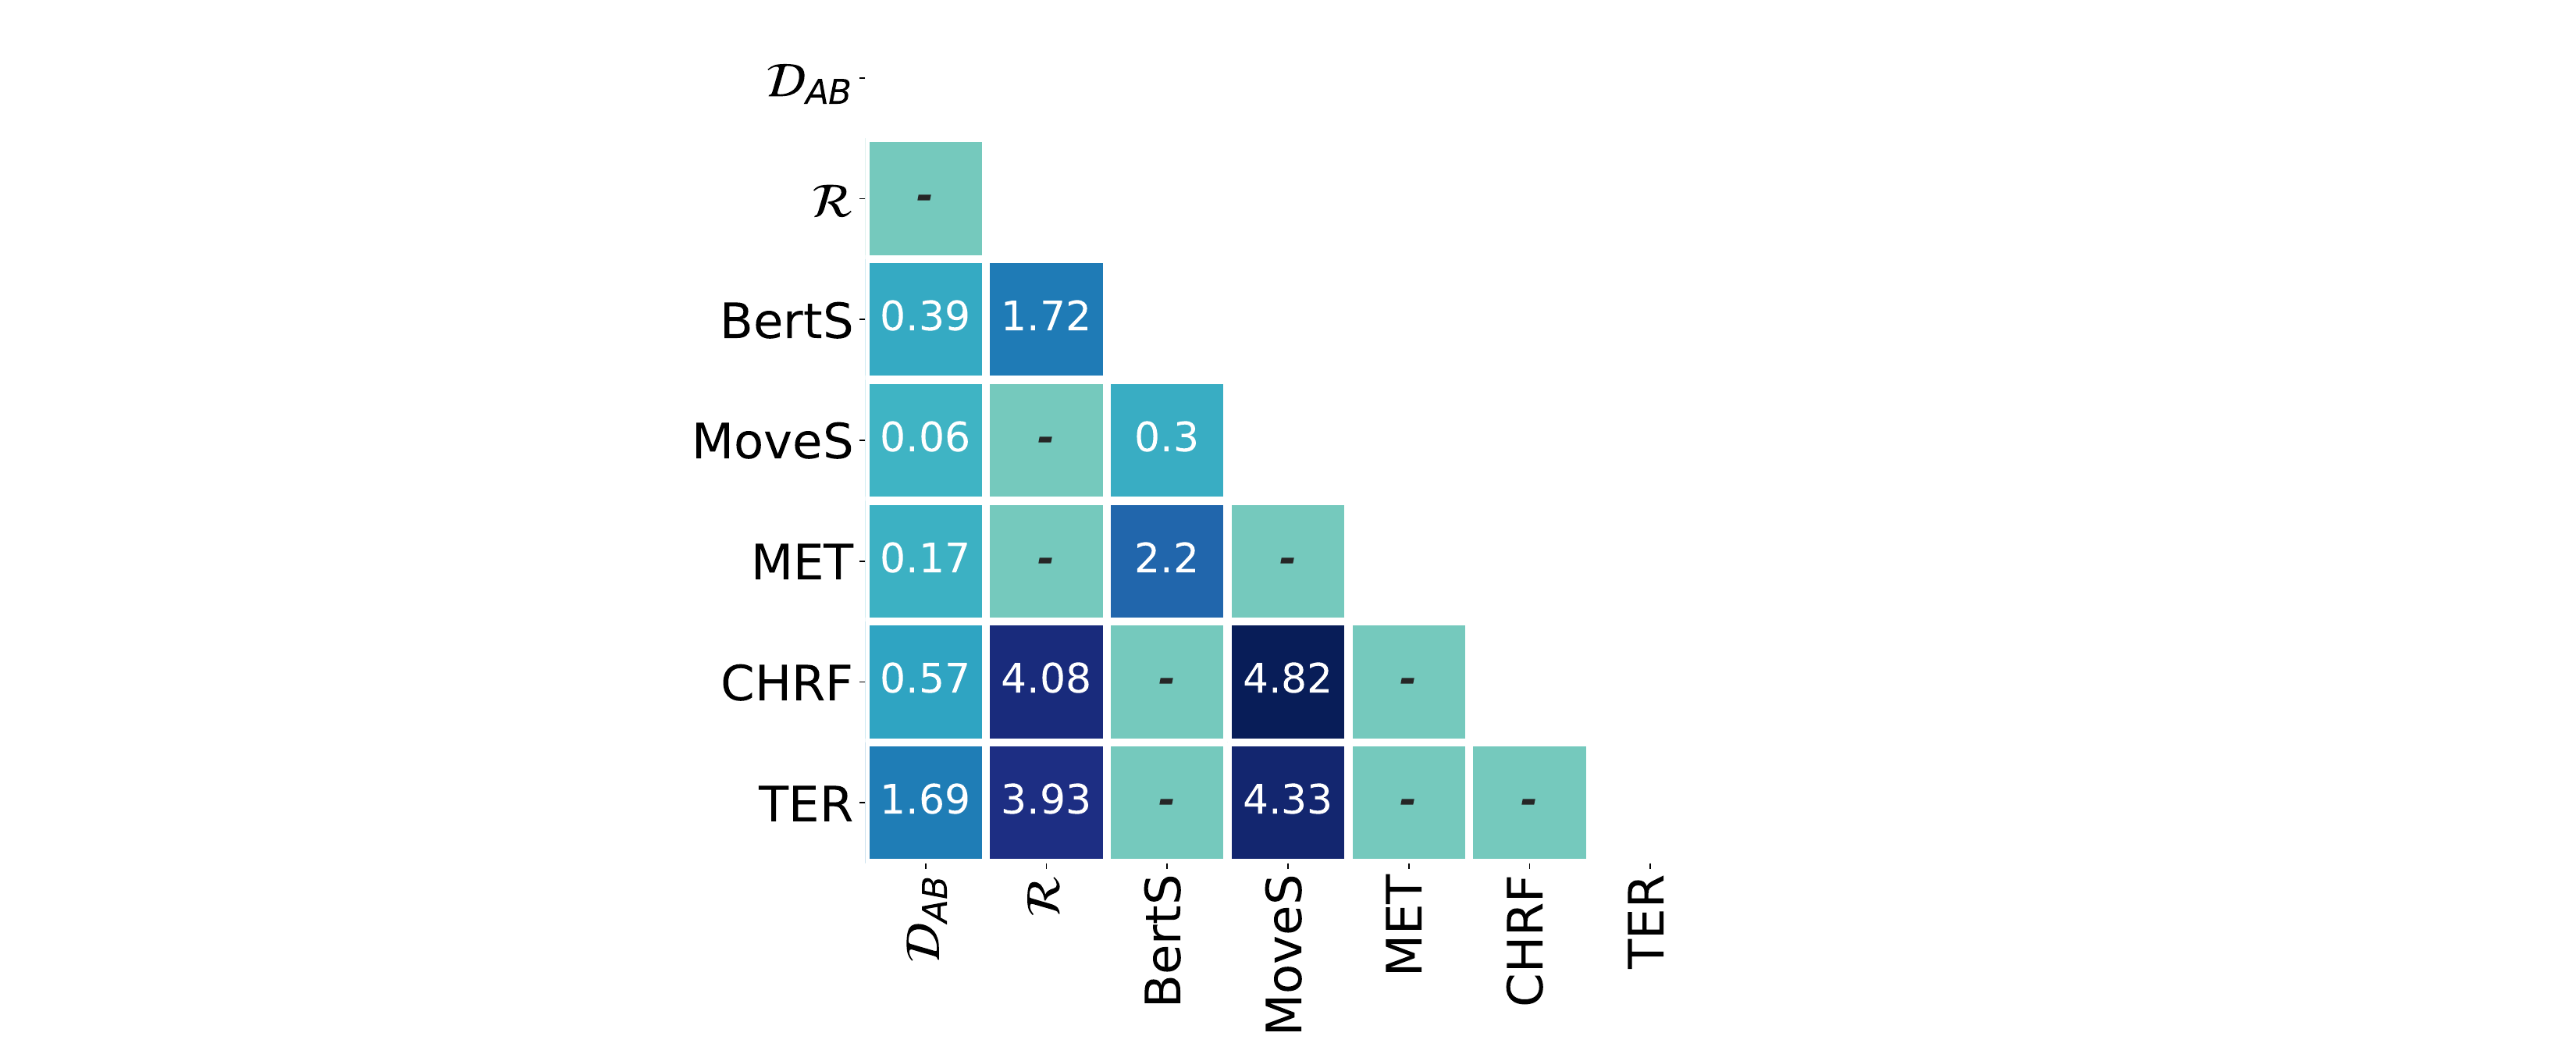}}
   \end{minipage}
      \begin{minipage}{0.18\textwidth}
      \vspace{.4cm}
     \centering
      \subfloat[Data C]{ \includegraphics[width=\linewidth]{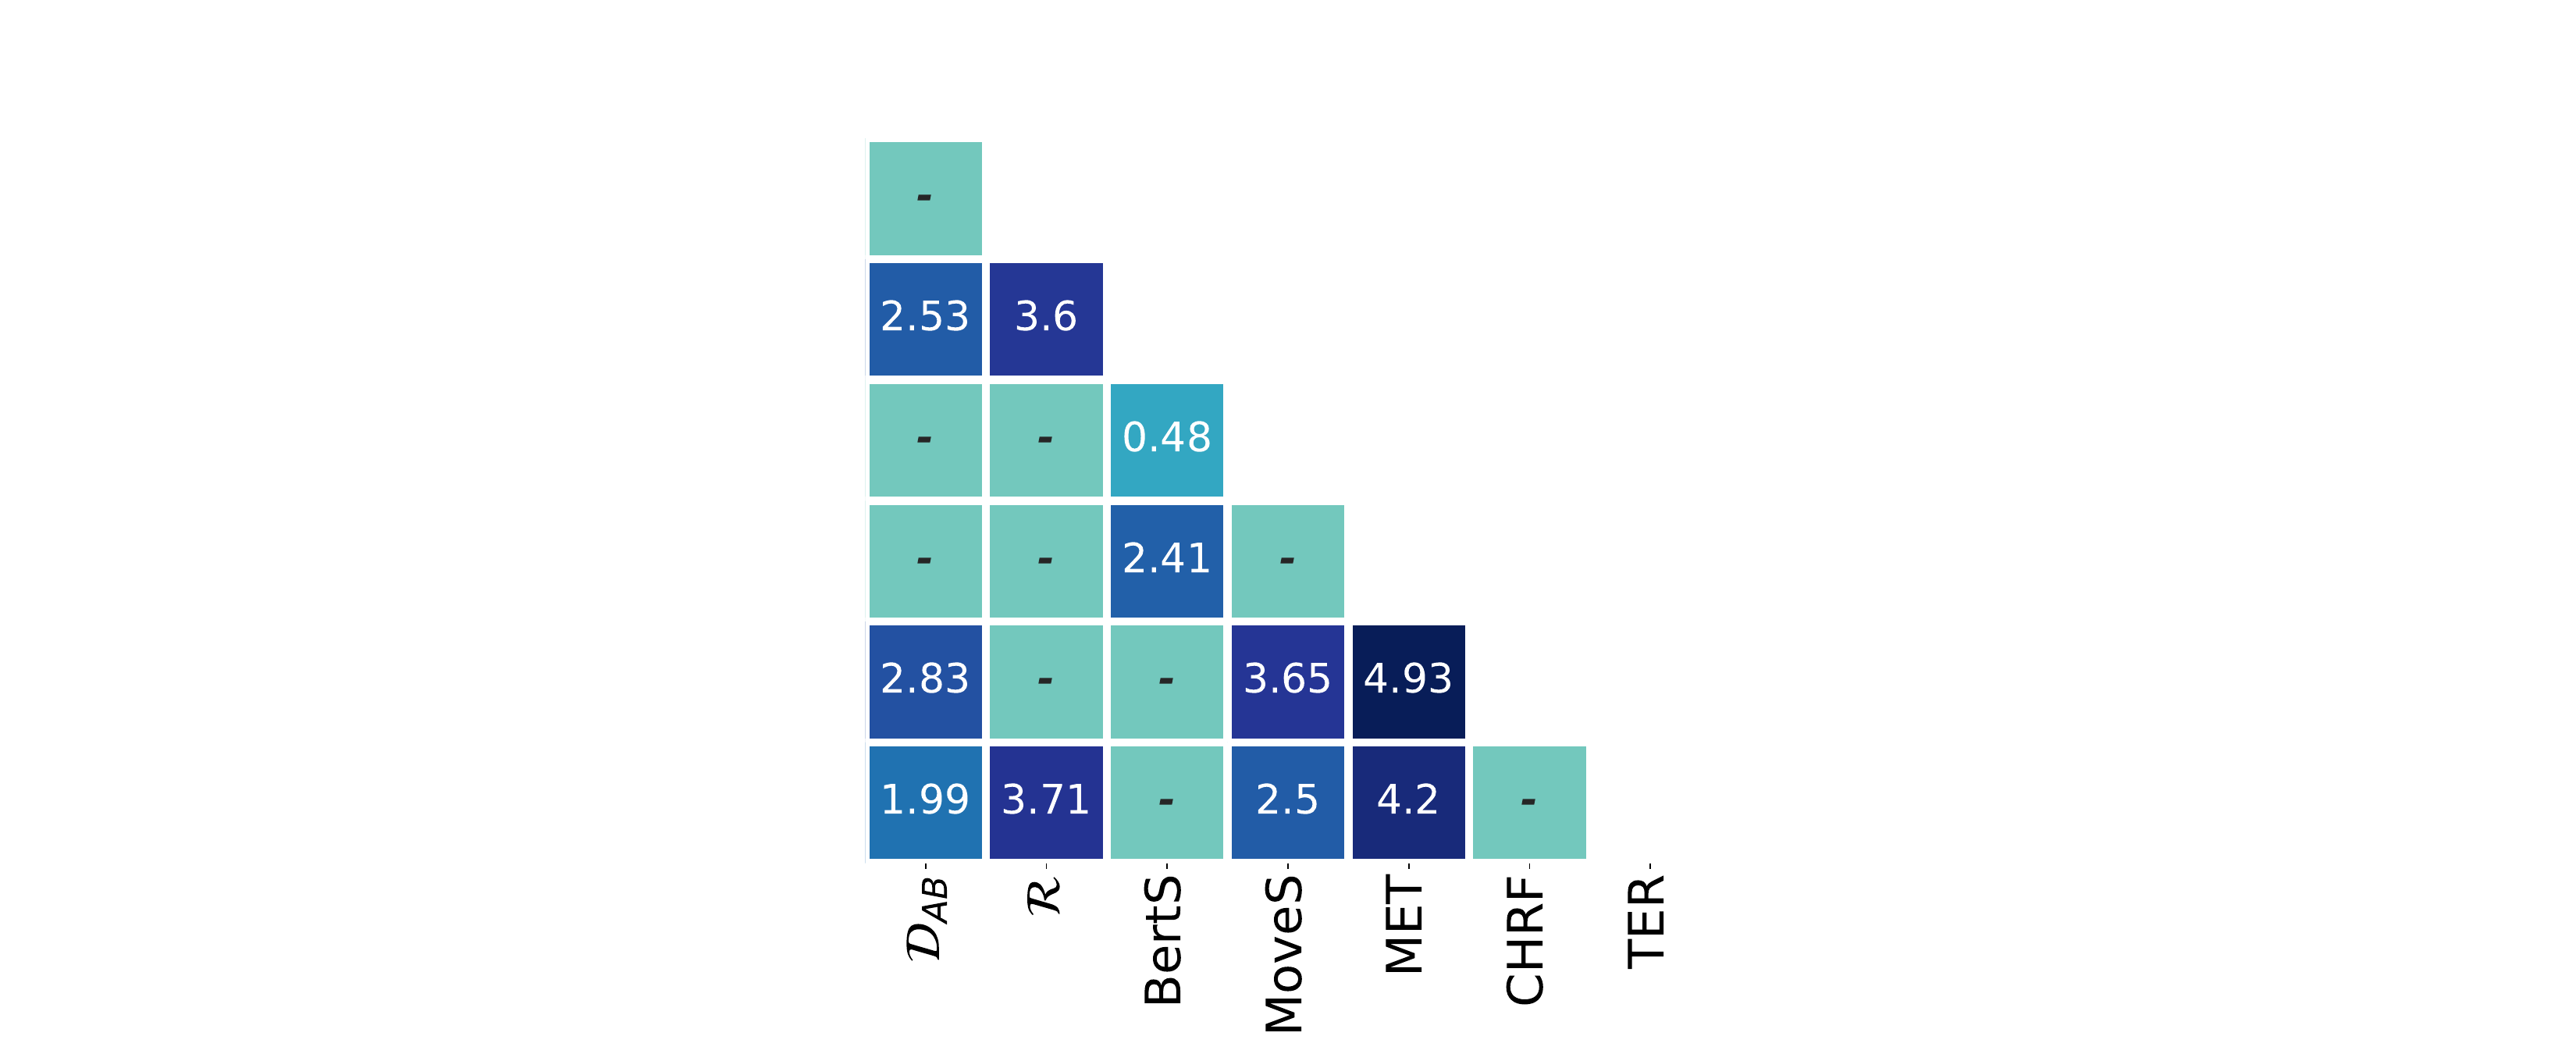}}
   \end{minipage}
      \begin{minipage}{0.18\textwidth}
      \vspace{.4cm}
     \centering
      \subfloat[Fluency]{ \includegraphics[width=\linewidth]{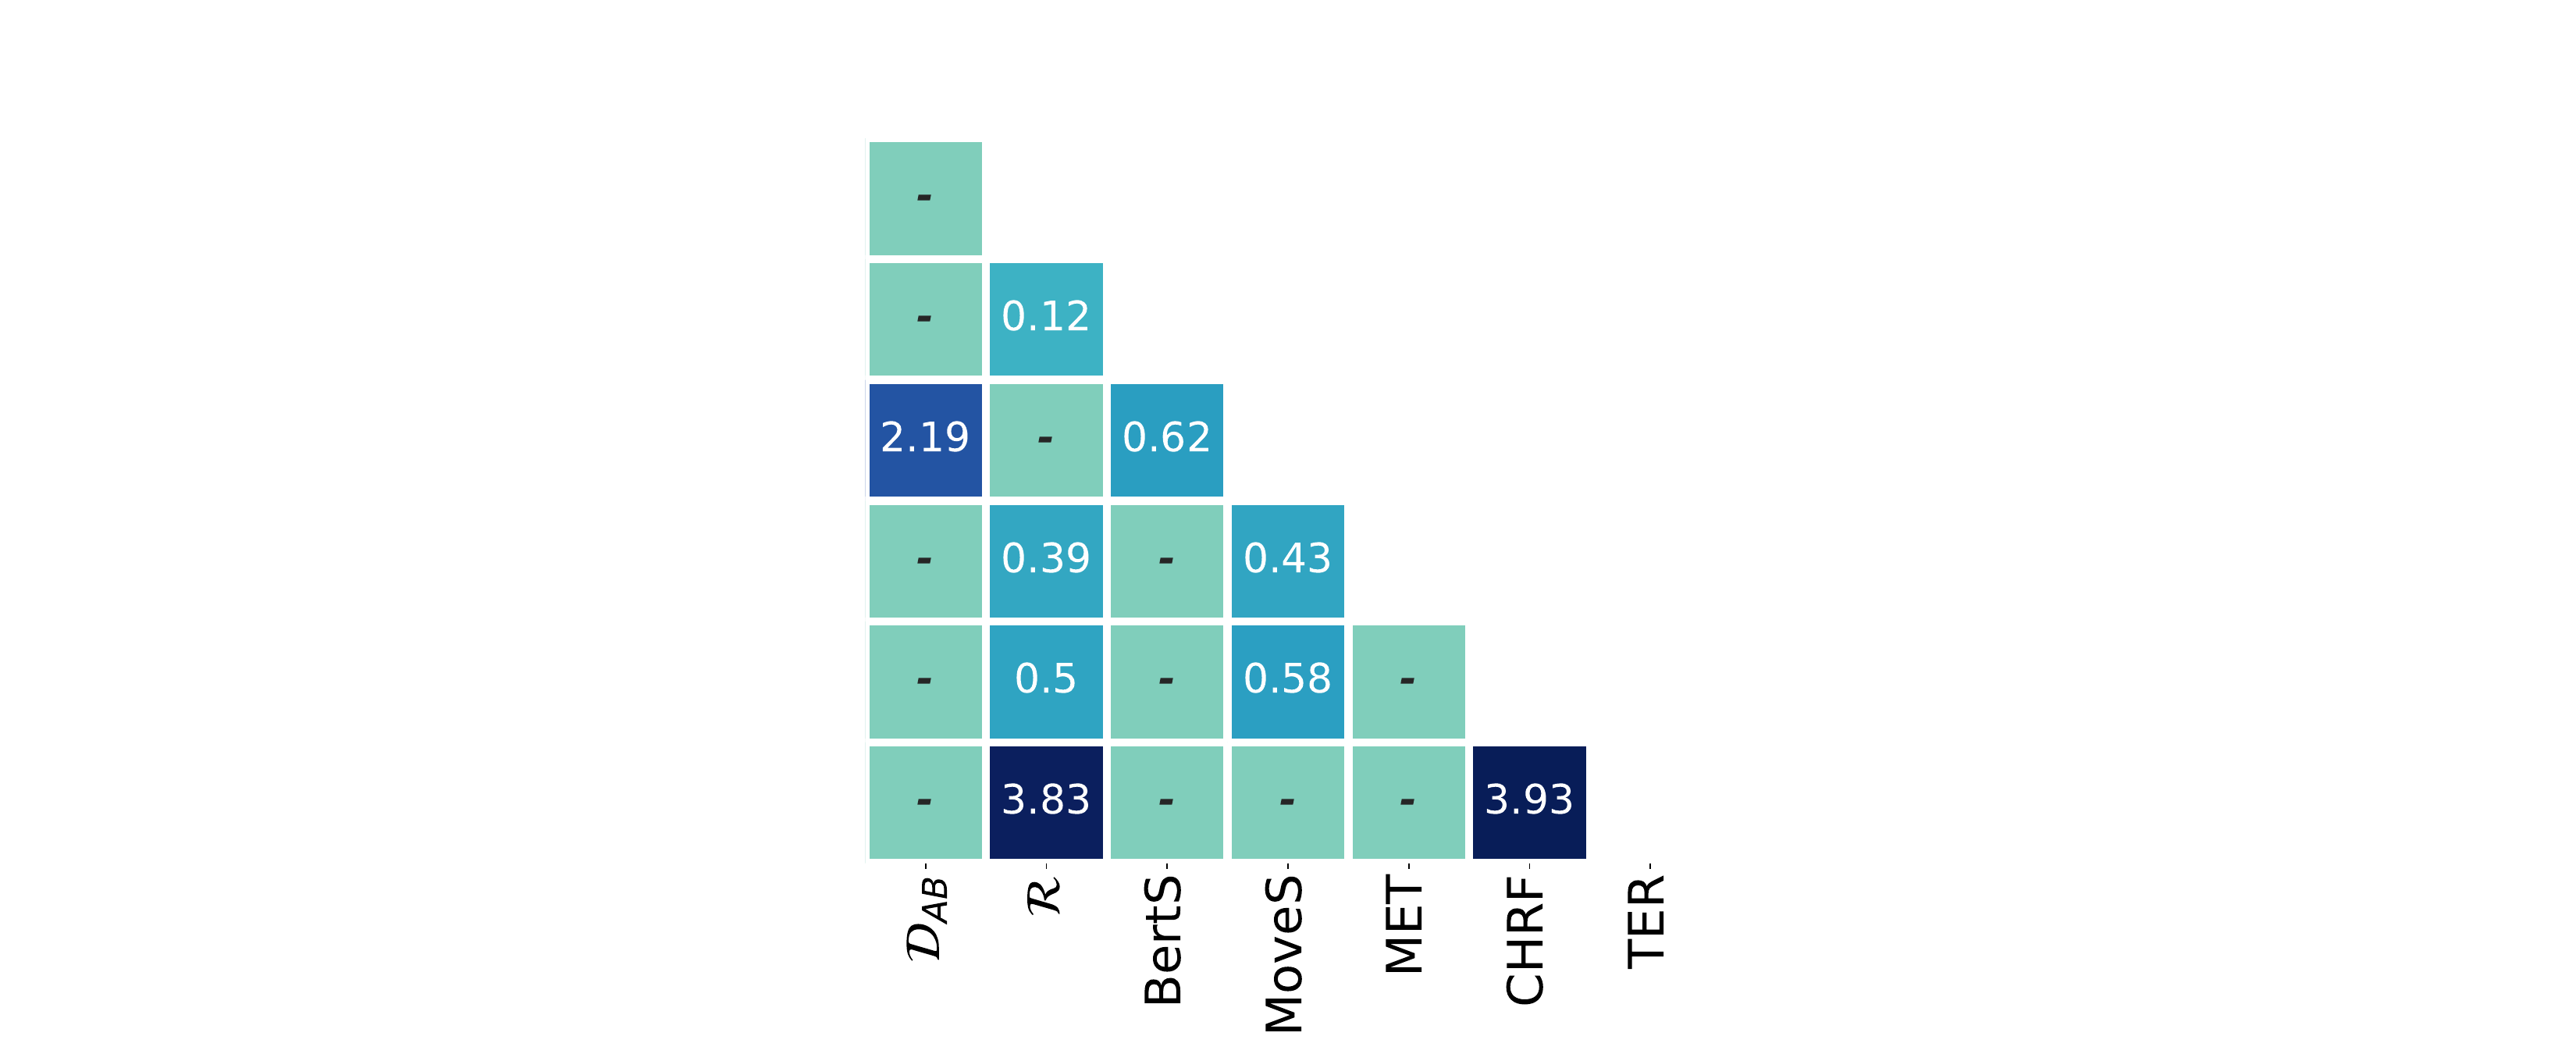}}
   \end{minipage}
      \begin{minipage}{0.18\textwidth}
      \vspace{.4cm}
     \centering
       \subfloat[Relev]{\includegraphics[width=\linewidth]{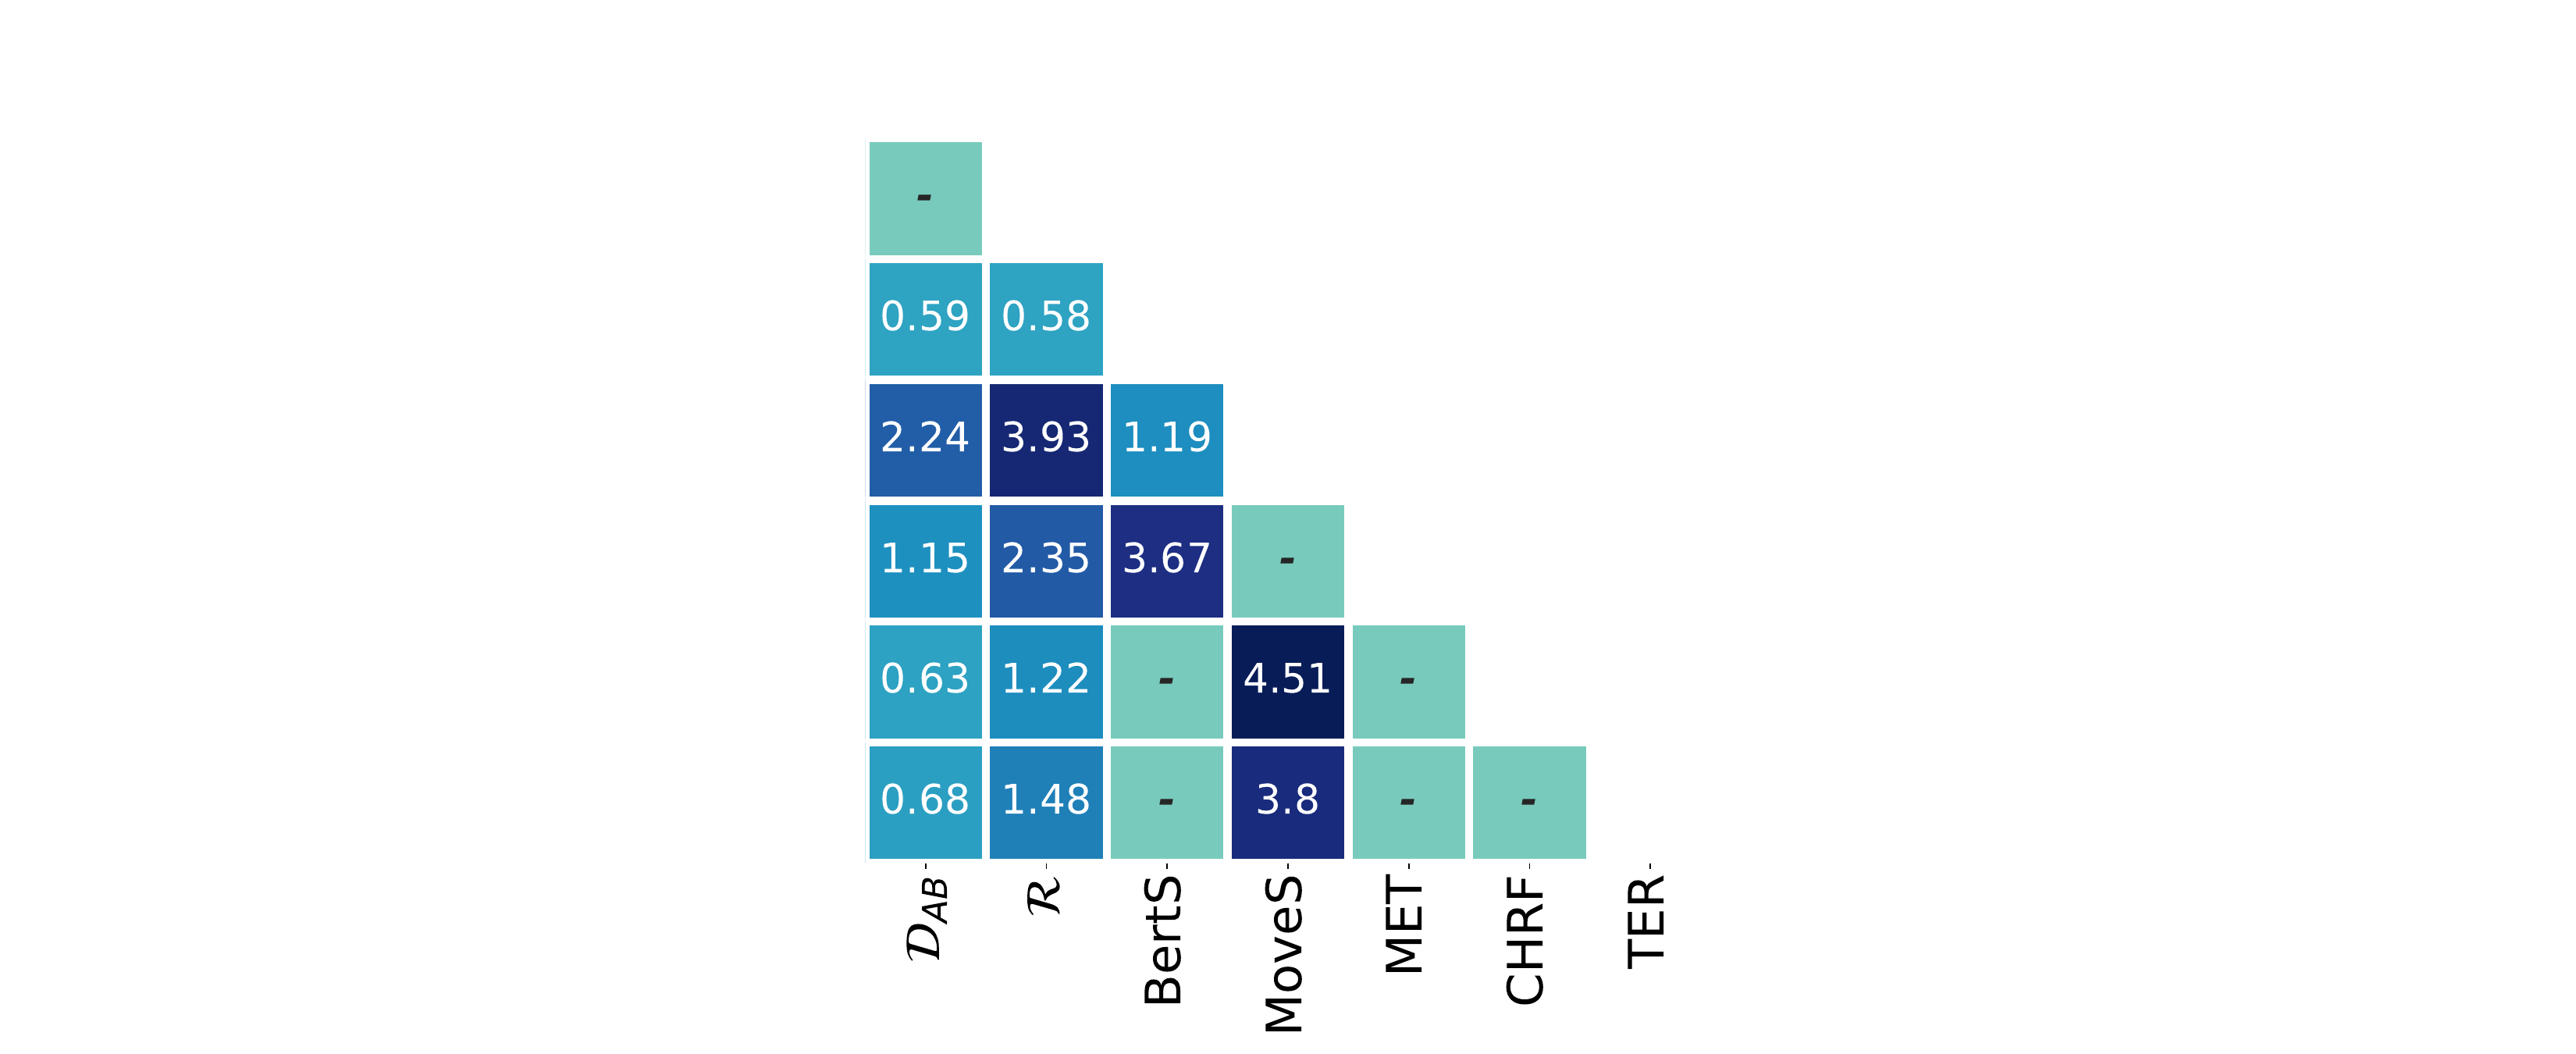}}
   \end{minipage}
      \begin{minipage}{0.18\textwidth}
      \vspace{.4cm}
     \centering
    \subfloat[Text S]{ \includegraphics[width=\linewidth]{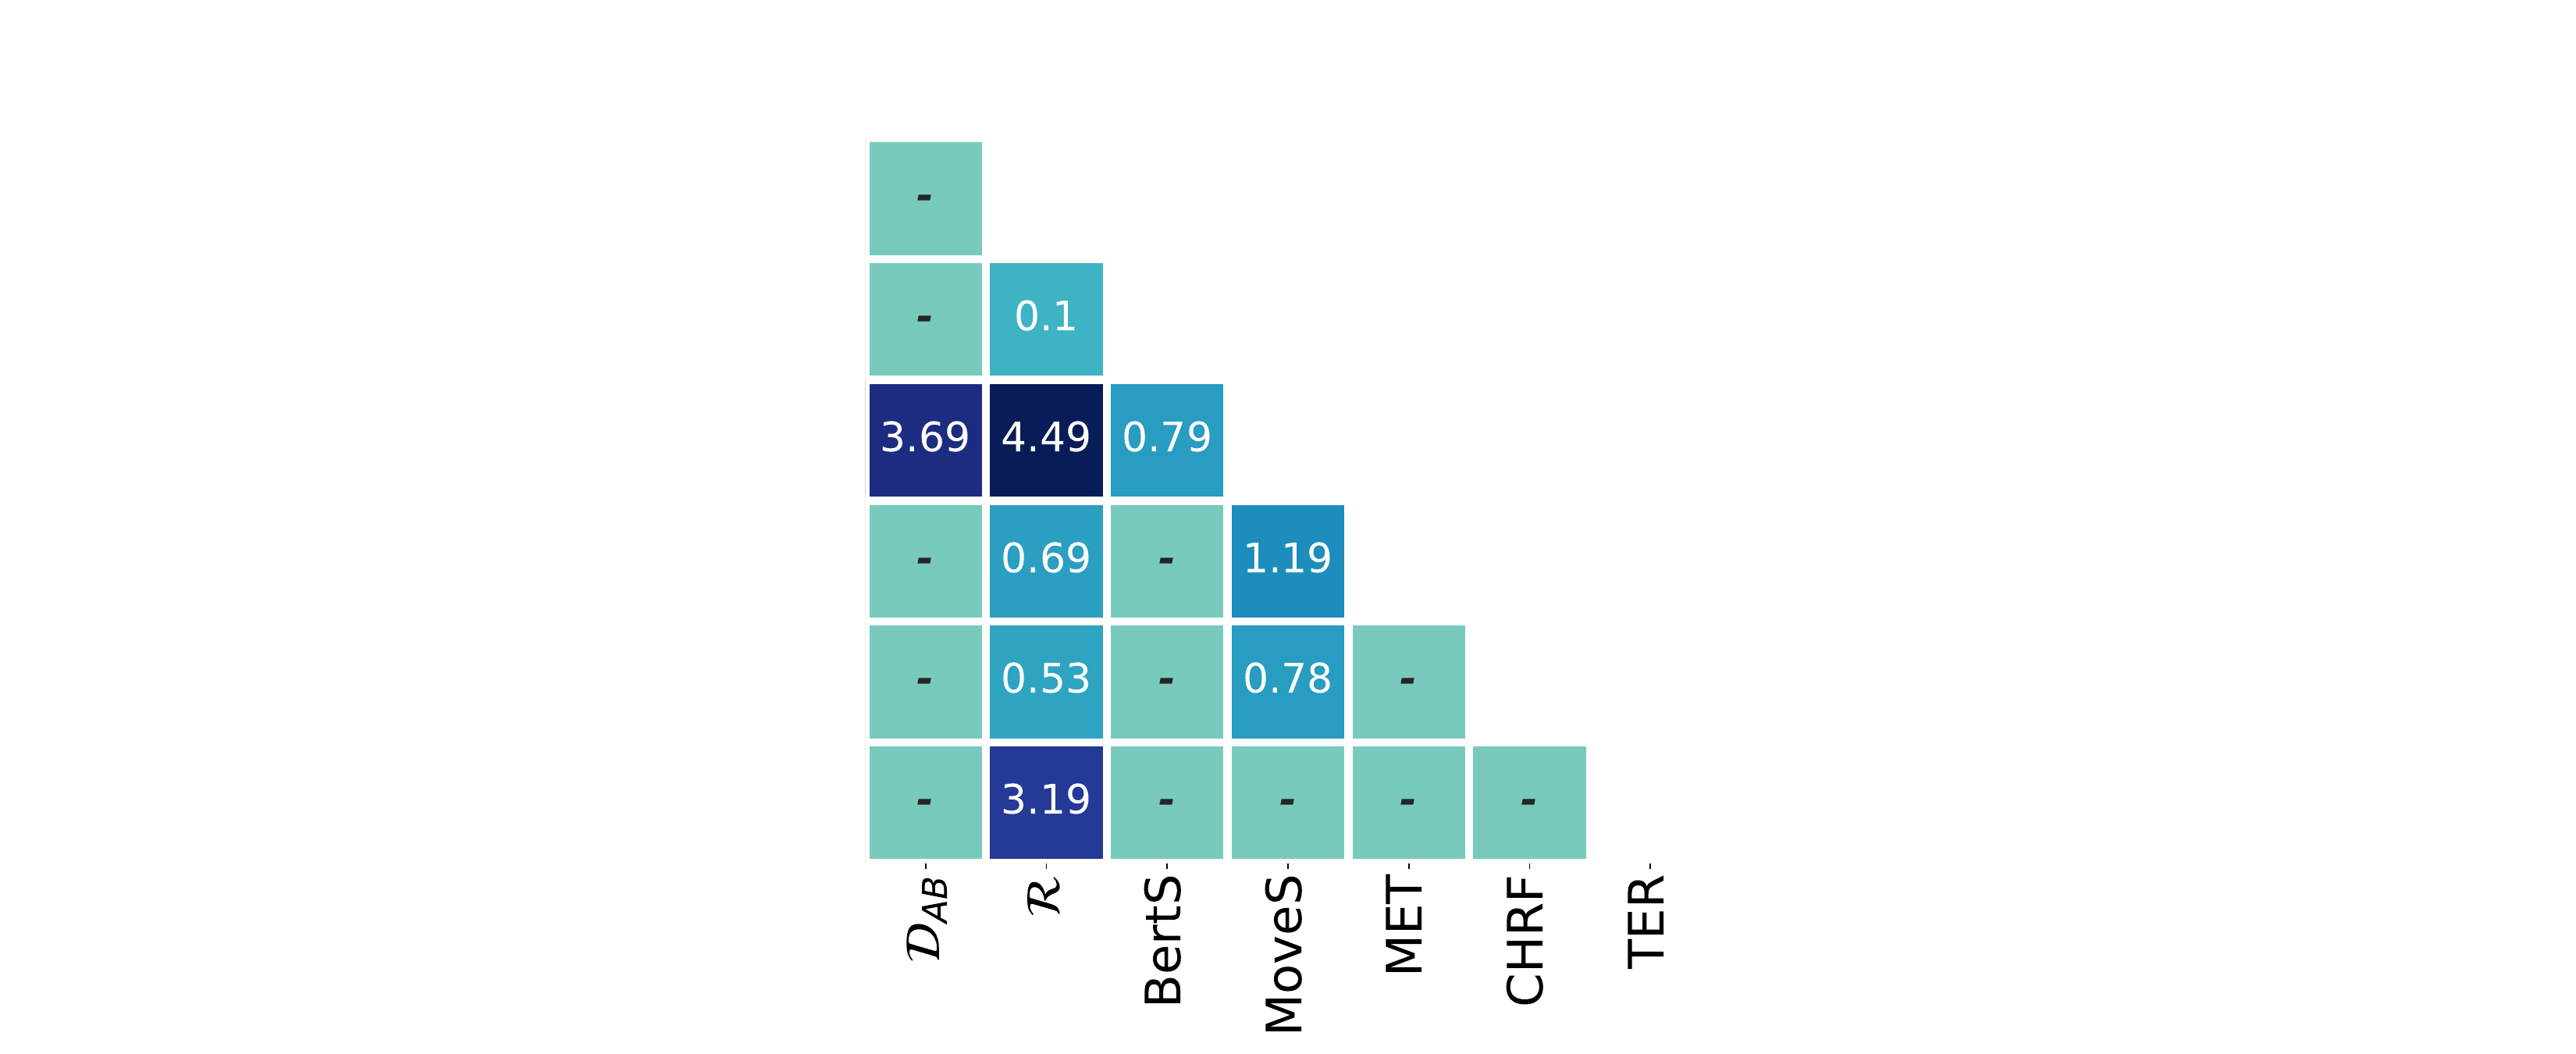}}
   \end{minipage}
   \caption{Results of William's Significance Test: the tested hypothesis is: ``is the increase of correlation significant''. For clarity and due to space constraints the p-values are truncated and multiply par 100. Only p-values that are lower than $5.00$ are displayed.}\label{fig:william}
\end{figure*}

\subsection{Complete results on Summarization}\label{ssec:complete_results_data2text}
We gather in \cref{fig:cnn_results_all}, the complete results on summarization. Due to space constraints, we did not report all the Spearman Correlation coefficients in the main paper. It is worth noting that our observations hold and the best performing metric is obtained with $\mathcal{D}_{AB}$. The Fisher-Rao distance, denoted by $R$, achieves
good performance in many scenarios and has the advantage
to be parameter-free.

\subsection{Complete results on Data2text Generation}\label{ssec:complete_results_data2text}
We gather in \cref{tab:web_nlg_sys}, the complete results on data2text generation. Due to space constraints, we did not report all the baselines in the main paper. 
\begin{table*}[]
    \centering

 \resizebox{\textwidth}{!}{\begin{tabular}{l|rrr|rrr|rrr|rrr|rrr|}\hline  
   &  \multicolumn{3}{c}{Correctness} & \multicolumn{3}{c}{Data Coverage} & \multicolumn{3}{c}{Fluency} &  \multicolumn{3}{c}{Relevance} &   \multicolumn{3}{c}{Text Structure} \\
  Metric &  $r$ &  $\rho$ & $\tau$  &  $r$ &  $\rho$ &  $\tau$ & $r$ &  $\rho$ &  $\tau$  &  $r$ &  $\rho$ &  $\tau$  & $r$ &  $\rho$ &  $\tau$  \\
\midrule               Correct &   100.0    &    100.0    &    100.0   &    97.6 &     85.2 &    73.3 &    80.0 &     81.1 &    61.6 &    99.1 &     89.7 &    75.0 &    80.1 &     80.8 &    60.0 \\                 
DataC &      85.2 &       97.6 &      73.3 &  100.0   &    100.0  &   100.0  &    71.8 &     51.7 &    38.3 &    96.0 &     93.8 &    81.6 &    71.6 &     51.4 &    36.6 \\               
Fluency &      81.1 &       80.0 &      61.6 &    71.8 &     51.7 &    38.3 &  100.0   &  100.0    &  100.0   &    77.0 &     61.4 &    46.6 &    99.5 &     99.7 &    98.3 \\                
Relev &      89.7 &       99.1 &      75.0 &    96.0 &     93.8 &    81.6 &    77.0 &     61.4 &    46.6 &  100.0   &  100.0    &  100.0   &    77.2 &     61.1 &    45.0 \\                 
TextS &      80.8 &       80.1 &      60.0 &    71.6 &     51.4 &    36.6 &    99.5 &     99.7 &    98.3 &    77.2 &     61.1 &    45.0 &  100.0   &  100.0    &   100.0  \\   \hline
$ \mathcal{D}_{AB}$ &      {88.8} &       \underline{\textbf{89.3}} &      \underline{\textbf{76.6}} &    \underline{\textbf{81.8}} &     \underline{\textbf{82.6}} &    \underline{\textbf{70.0}} &    86.6 &     92.0 &    76.6 &    \underline{\textbf{89.8}} &     \underline{\textbf{87.9}} &    \underline{{73.3}} &    86.6 &     91.4 &    75.0 \\ 
$ \mathcal{D}_\alpha$ &      {88.8} &       \underline{\textbf{89.3}} &      \underline{\textbf{76.6}} &    \underline{\textbf{81.8}} &     \underline{\textbf{82.6}} &    \underline{\textbf{70.0}} &    86.6 &     92.0 &    76.6 &   \underline{ \textbf{89.8}} &     \underline{\textbf{87.9}} &    \underline{{73.3}} &    86.6 &     91.4 &    75.0 \\   
$ \mathcal{D}_\beta$ &      81.4 &       50.0 &      71.6 &    48.4 &     79.7 &    65.0 &    44.8 &     84.7 &    76.6 &    49.3 &     72.3 &    60.0 &    48.0 &     83.8 &    75.0 \\      
$ \mathcal{L}_1$ &      75.2 &       33.8 &      61.6 &    32.4 &     53.8 &    40.0 &    22.7 &     83.5 &    73.3 &    32.2 &     57.9 &    45.0 &    25.6 &     83.2 &    71.6 \\  
$ \mathcal{L}_2$ &      67.0 &       21.9 &      56.6 &    21.6 &     37.9 &    33.3 &    11.9 &     75.2 &    58.3 &    20.1 &     43.8 &    38.3 &    14.8 &     75.5 &    60.0 \\ 
$ \mathcal{L}_\infty$ &      63.2 &       33.0 &      46.6 &    30.4 &     36.4 &    26.6 &    67.6 &     65.0 &    46.6 &    29.1 &     49.1 &    35.0 &    67.2 &     65.2 &    46.6 \\        
$ \mathcal{R}$ &      \underline{\textbf{89.7}} &       86.0 &      75.0 &    78.7 &     70.5 &    51.6 &    \underline{\textbf{93.3}} &     \underline{\textbf{95.7}} &    \underline{\textbf{85.3}} &   87.6 &     84.4 &    70.0 &    \underline{\textbf{92.4}} &     \underline{93.8} &    \underline{81.6} \\                   
JS &      79.4 &       81.1 &      70.0 &    69.3 &     75.5 &    60.0 &    89.4 &     91.4 &    75.0 &    81.7 &     70.5 &    60.0 &    91.9 &     91.1 &    73.3 \\ \hline                
BertS &      \underline{85.5} &       83.4 &      \underline{73.3} &    
74.7 &     \underline{68.2} &    53.3 &    
\underline{92.3} &     \underline{95.5} &    \underline{85.0} &    
\underline{83.3} &     \underline{79.4} &    \underline{65.0} &    
\underline{91.9} &     \underline{\textbf{95.0}} &    \underline{\textbf{83.3}} \\       
MoverS &      84.1 &       \underline{84.1} &      \underline{73.3} &    
\underline{78.7} &     66.2 &    \underline{53.3} &    
91.2 &     92.1 &    78.3 &    
82.1 &     77.4 &    65.0 &    
90.1 &     91.4 &    76.3 \\\hline  
BLEU &      77.6 &       66.3 &      60.0 &    
55.7 &     50.2 &    36.6 &    
\underline{89.4} &     90.5 &    78.3 &    
63.0 &     65.2 &    51.6 &    
{88.5} &     89.1 &    76.6 \\
R-1 &      80.6 &       65.0 &      65.0 &    61.1 &     \underline{59.6} &    \underline{48.3} &    
76.5 &     76.3 &    60.3 &    
64.3 &     \underline{69.2} &    56.7 &    
75.9 &     77.5 &    58.3 \\
R-2 &      73.6 &       63.3 &      58.3 &    54.7 &     43.1 &    35.0 &    
86.4 &     81.9 &    63.4 &   
62.0 &     60.8 &    46.7 &    
86.5 &     80.5 &    61.7 \\
R-WE &      60.9 &       73.4 &      60.0 &    40.2 &     58.2 &    40.1 &    
61.4 &     84.7 &    61.3 &    
49.9 &     64.1 &    48.3 &    
60.2 &     85.9 &    60.0 \\
METEOR &      \underline{86.5} &       \underline{66.3} &      \underline{70.0} &    
\underline{77.3} &     50.2 &    46.6 &    
86.7 &     90.5 &    78.3 &    
\underline{82.1} &     65.2 &    58.6 &    
86.2 &     89.1 &    76.6 \\
TER &      79.6 &       78.3 &      58.0 &    69.7 &     58.2 &    38.0 &    89.1 &     \underline{93.5} &    \underline{80.0} &    75.0 &     70.2 &    \underline{\textbf{77.6}} &    \underline{89.5} &     \underline{91.1} &    \underline{78.6} \\
\bottomrule\end{tabular}}
\caption{Correlation at the system level with human judgement along five different axis: correctness, data coverage, fluency, relevance and text structure for the WebNLG task. Best results by group are underlined, overall best results are bolted.}
    \label{tab:web_nlg_sys}
\end{table*}

\subsection{Complete Results on Score Distribution}\label{ssec:score_distrib_appendix}
We gather in \cref{fig:score_distribation} the score distribution on the summarization dataset. It is worth noting that for these experiments we have scaled the divergences between 0 and 1 and we have considered 1 - \texttt{InfoLM}.

\section{Additional details on the datasets}\label{sec:additionnal_dataset_details}
\subsection{Summarization}\label{sec:additional_details_summarization}
The summarization dataset CNN can be found in \url{https://github.com/neulab/REALSumm} and no preprocessing has been applied. Specifically, the summaries have been generated using 14 abstractive systems \cite{zhong2020extractive,wang2020heterogeneous,zhong2019searching,liu2019text,zhou2018neural,narayan2018ranking,dong2019unified,kedzie2018content,zhou2018neural} and 11 extractive systems \cite{see2017get,chen2018fast,raffel2019exploring,gehrmann-etal-2018-bottom,dong2019unified,liu2019text,lewis2019bart,yoon2020learning}.
\\\textbf{Pyramide Score.} The Pyramide score, which was inspired from work in reading comprehension (see \citet{beck1991revising}) is a scoring procedure to assess the semantic content in the scope of summarization. The manual methods are based on the concept of Summary Content Units (SCUs) which groups sentences from different summaries. grouping if they carry the same content.

\subsection{Data2text}\label{sec:additional_details_data2text}
The goal of the WebNLG challenge is to develop efficient Knowledge Base Verbalizers \cite{gardent2017creating,perez2016building}(\textit{i.e} generation algorithms that can verbalise knowledge base fragments) and thus handle complex interaction that can occur during the micro-planning phase when generating sentences \cite{ferreira2018enriching}. Details on the WebNLG2020 task are given in \citet{ferreira20202020}. The dataset is composed of generated sentences coming from 15 different systems using various approaches such as symbolic approaches or neural-based systems. All data are freely available on GitHub \url{https://gitlab.com/shimorina/webnlg-dataset/-/tree/master/release_v3.0} and no preprocessing has been applied. For the dataset, they use the RDF format which is a widely used format for many datasets such as LinkedGeoData \url{http://linkedgeodata.org/About}, FOAF \url{http://www.foaf-project.org/} or MusicBrainz \url{https://musicbrainz.org/}. extracted from DBpedia \cite{auer2007dbpedia}.

\subsection{Limitations}\label{sec:additional_details_data2text}
We have evaluate our metrics on text only datasets. Future work will also investigate robustness of the metric to type of texts (\textit{e.g} spoken text \cite{dinkar2020importance,chapuis2021code,chapuis2020hierarchical}) and the extension to multimodal setting \cite{colombo2021improving,garcia2019token} and other type of task (\textit{e.g} related to dialog \cite{colombo2021beam} and affect driven text generation \cite{colombo2019affect,witon2018disney} and intend generation \cite{mehri2020example} with dialog acts \cite{colombo2020guiding}).

\subsection{Metric Choices}
 Several revised versions of \texttt{BLEU} \cite{doddington2002automatic,galley2015deltableu} and \texttt{METEOR} \cite{denkowski2014meteor,guo-hu-2019-meteor} have been proposed in recent years. For our implementation we choose to use SACREBLEU \cite{sacrebleu}. Similarly, a plethora of ROUGE extension have been proposed (\cite{ganesan2018rouge,shafieibavani2018graph}) but in our work we choose to work with \texttt{ROUGE-1}, \texttt{ROUGE-2} and \texttt{ROUGE-WE}. For the BERT based metrics, we choose to rely on the most popular although several alternatives exists (\textit{e.g.} \texttt{SENTENCE-MOVER} \cite{clark-etal-2019-sentence})

\begin{figure*}\vspace{-0.5cm}
\centering
\resizebox{\textwidth}{!}{\begin{tabular}{cccc}
\subfloat[Abs - Text]{\includegraphics[trim=100 20 0 0,width = 1.5in]{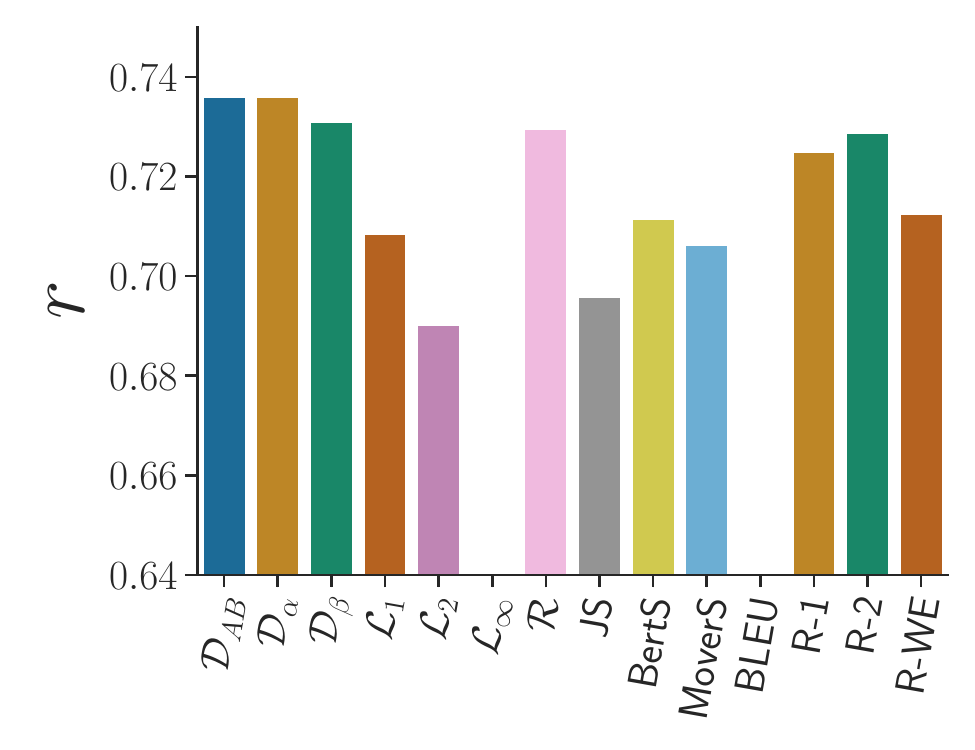}} &
\subfloat[Ext - Text]{\includegraphics[trim=50 20 0 0,width = 1.5in]{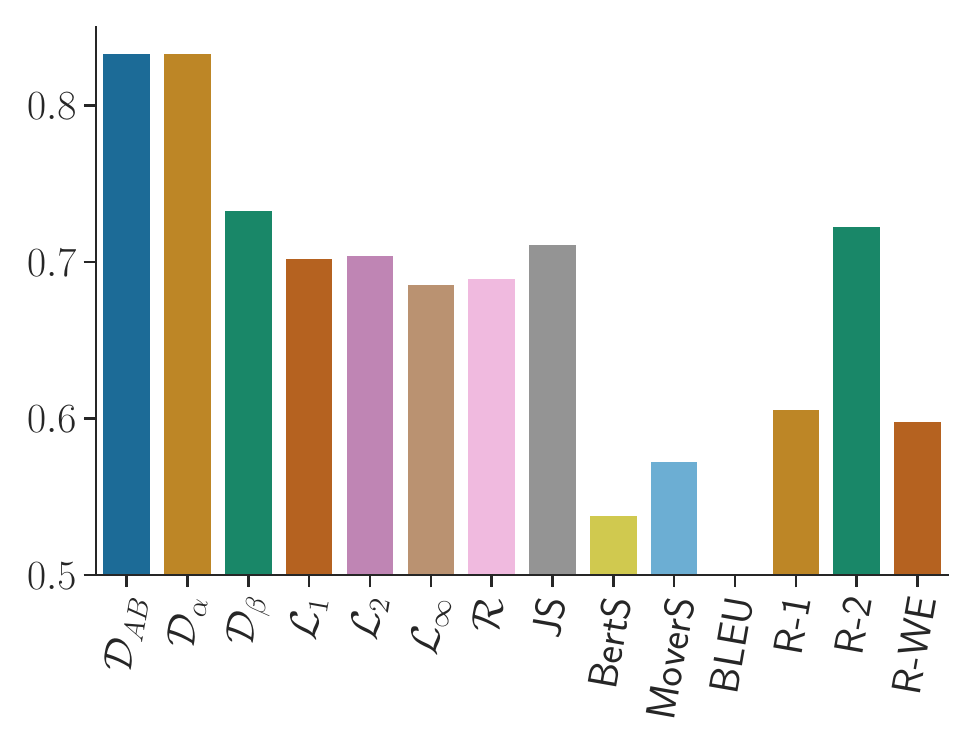}} &
\subfloat[Abs - Sys]{\includegraphics[trim=50 20 0 0,width = 1.5in]{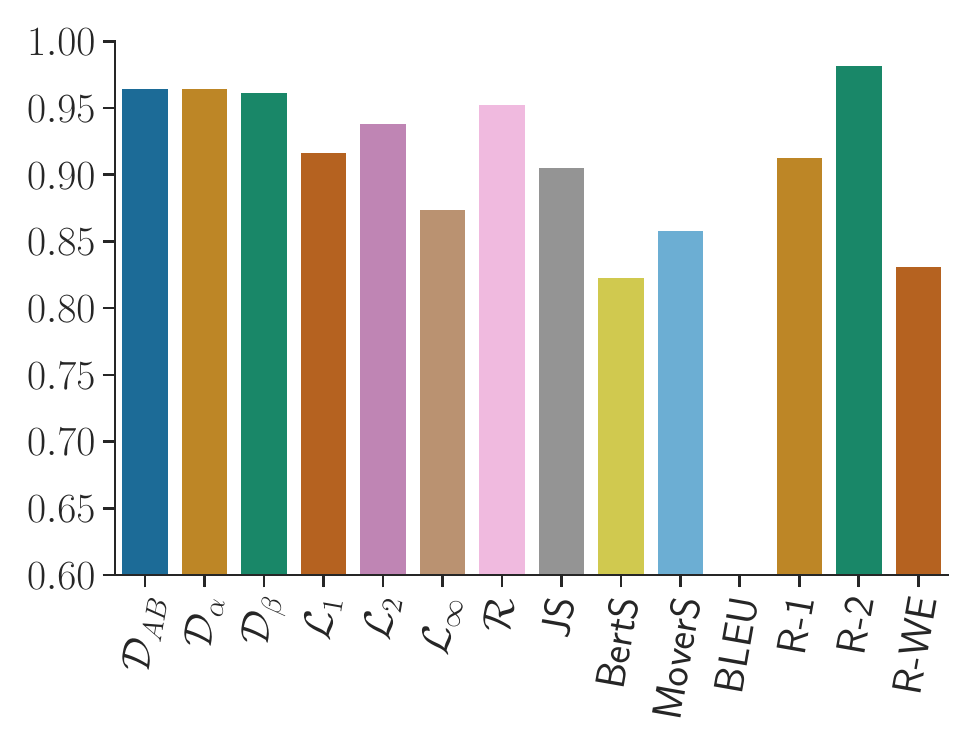}} &
\subfloat[Ext - Sys]{\includegraphics[trim=50 20 0 0,width = 1.5in]{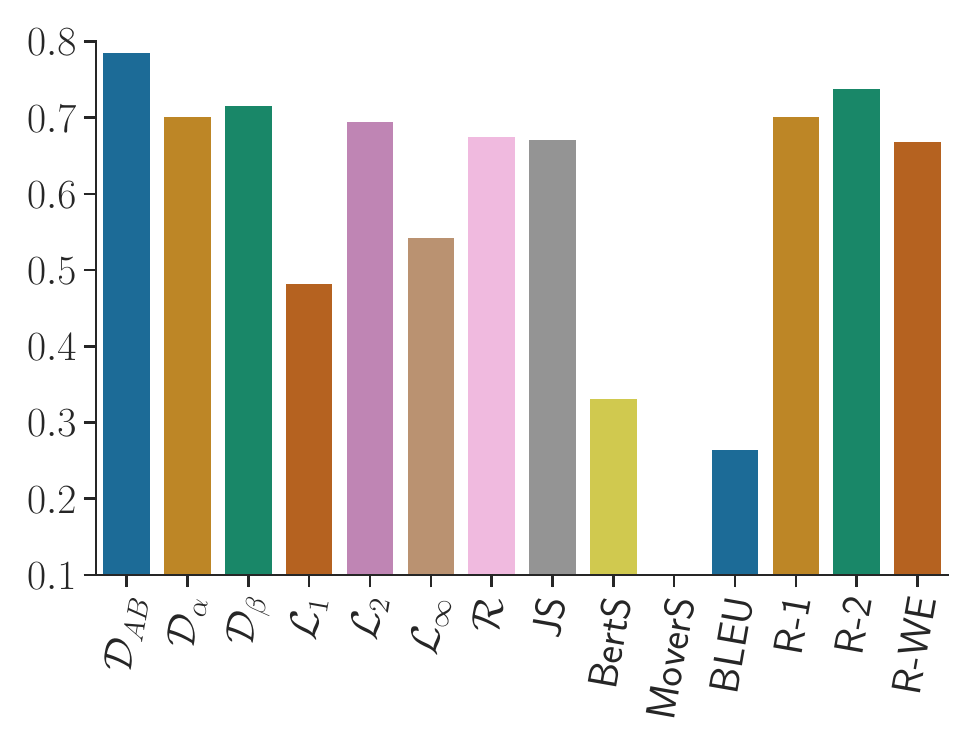}}\\\vspace{-.15cm}
\subfloat[Abs - Text]{\includegraphics[trim=100 20 0 0,width = 1.5in]{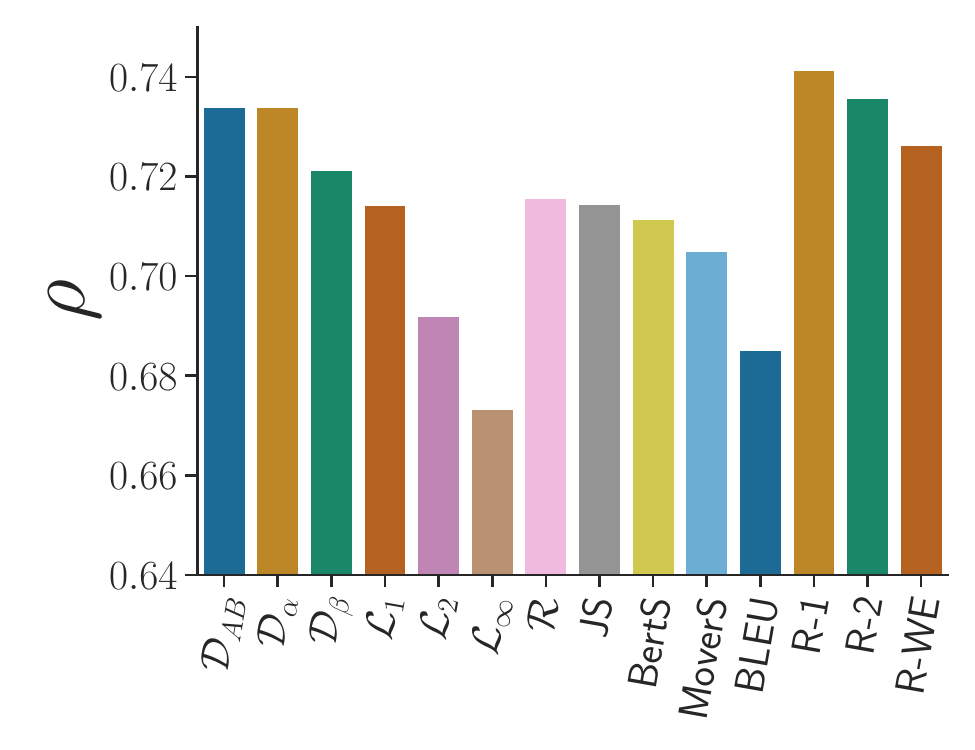}} &
\subfloat[Ext - Text]{\includegraphics[trim=50 20 0 0,width = 1.5in]{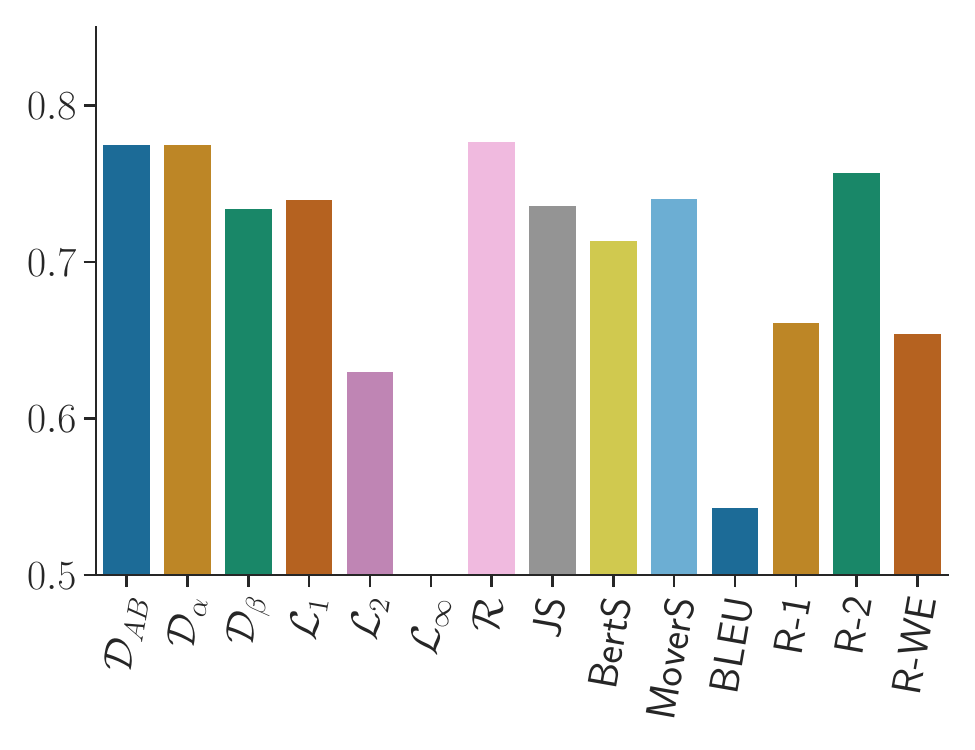}}&
\subfloat[Abs - Sys]{\includegraphics[trim=50 20 0 0,width = 1.5in]{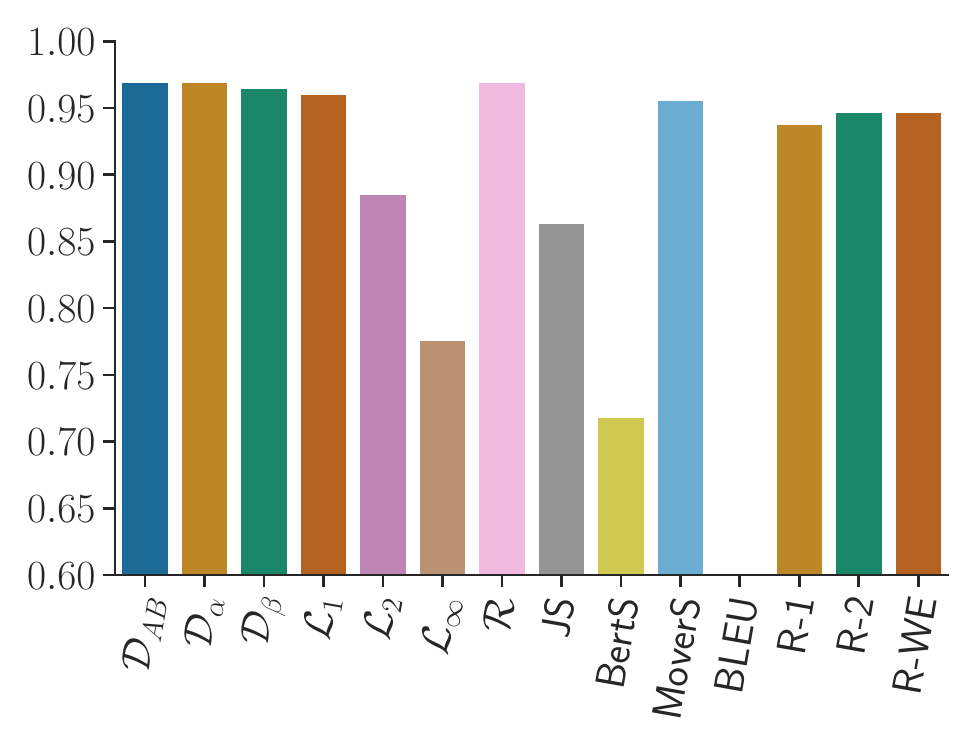}} &
\subfloat[Ext - Sys]{\includegraphics[trim=50 20 0 0,width = 1.5in]{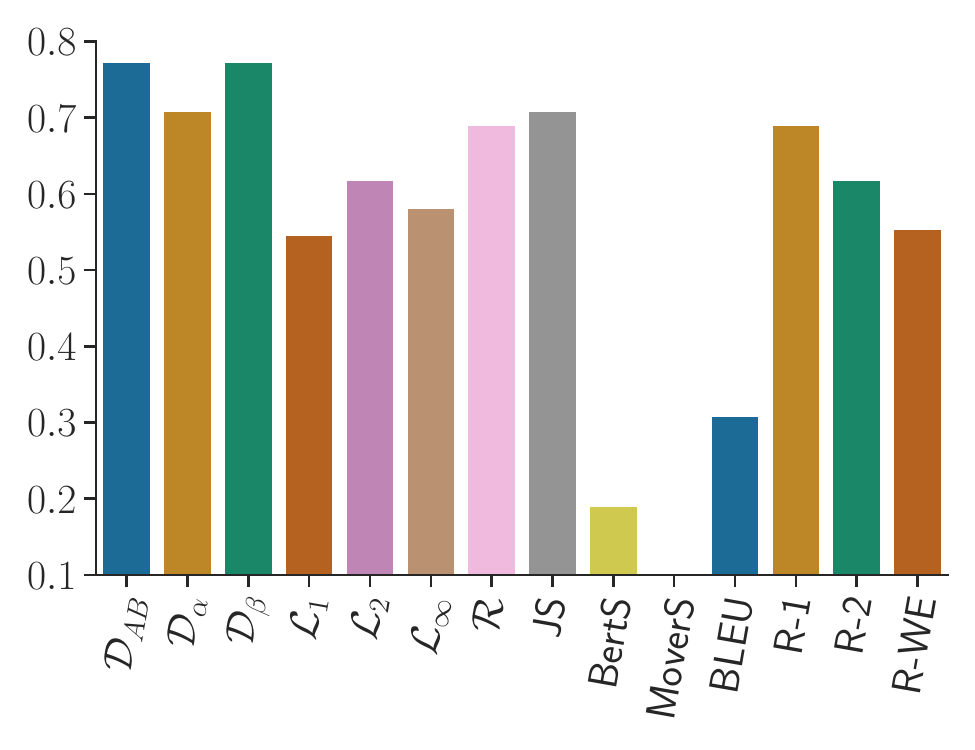}}\\\vspace{-.15cm}
\subfloat[Abs - Text]{\includegraphics[trim=100 20 0 0,width = 1.5in]{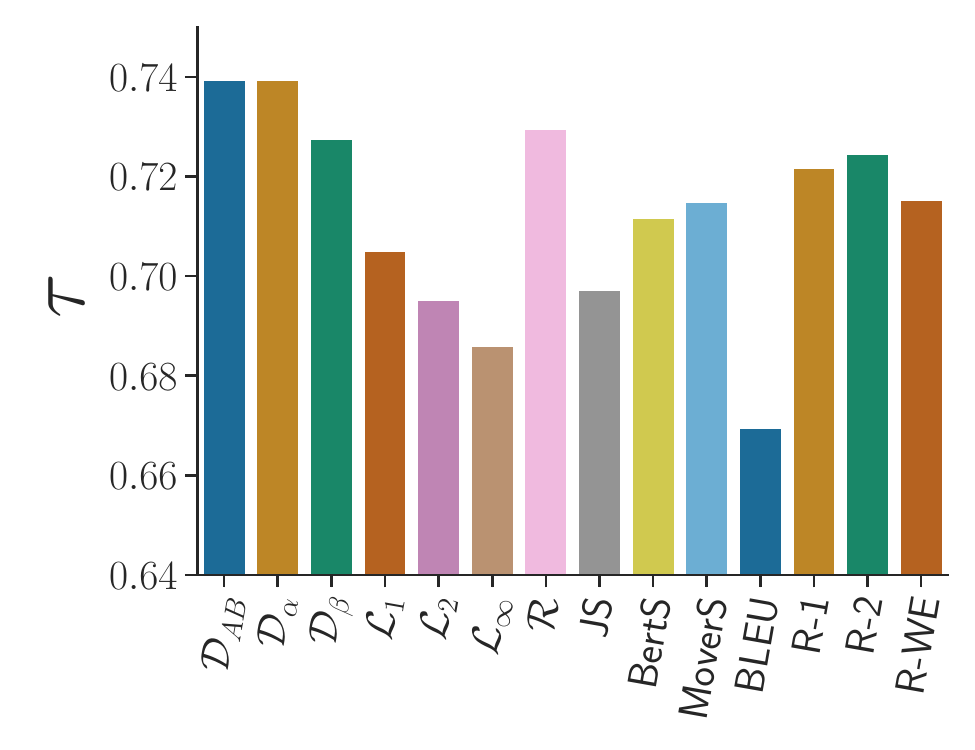}} &
\subfloat[Ext - Text]{\includegraphics[trim=50 20 0 0,width = 1.5in]{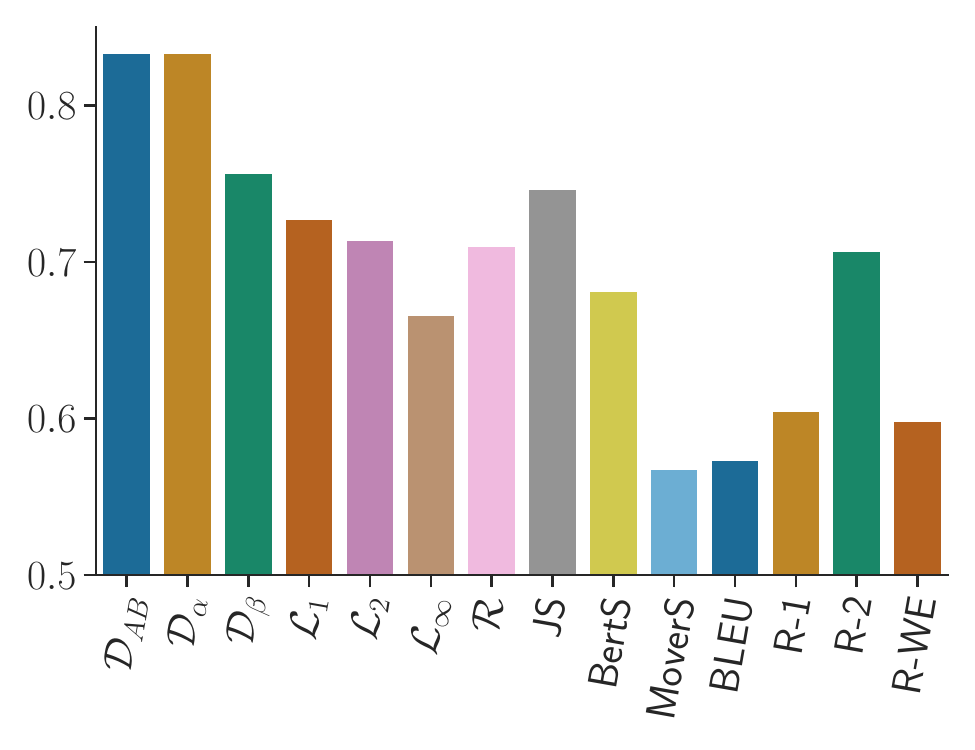}} &
\subfloat[Abs - Sys]{\includegraphics[trim=50 20 0 0,width = 1.5in]{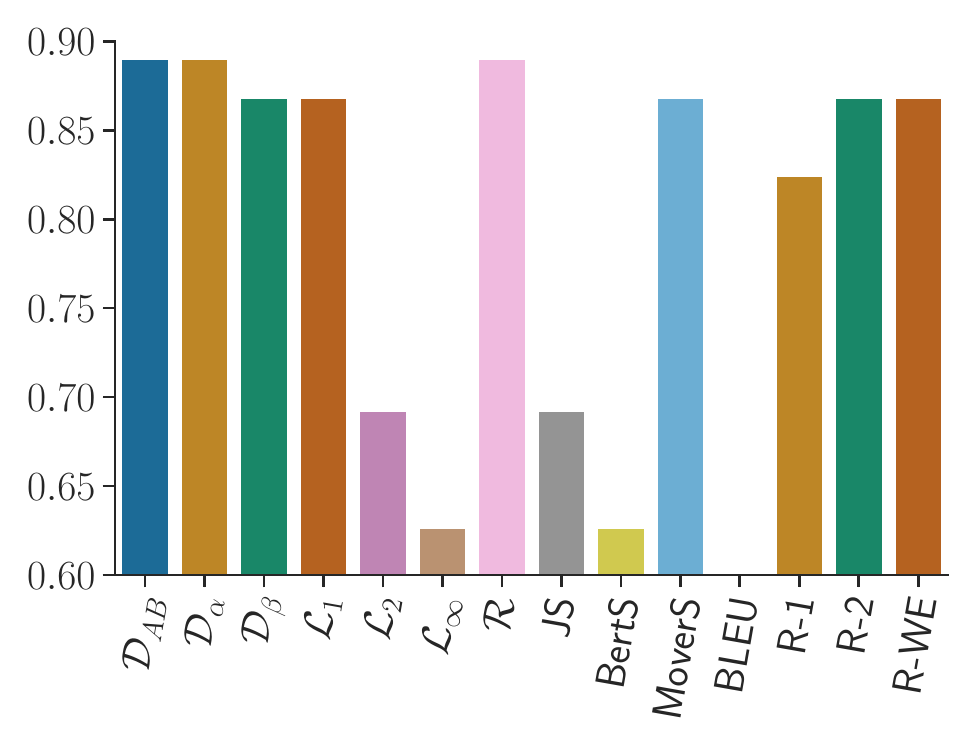}} &
\subfloat[Ext - Sys]{\includegraphics[trim=50 20 0 0,width = 1.5in]{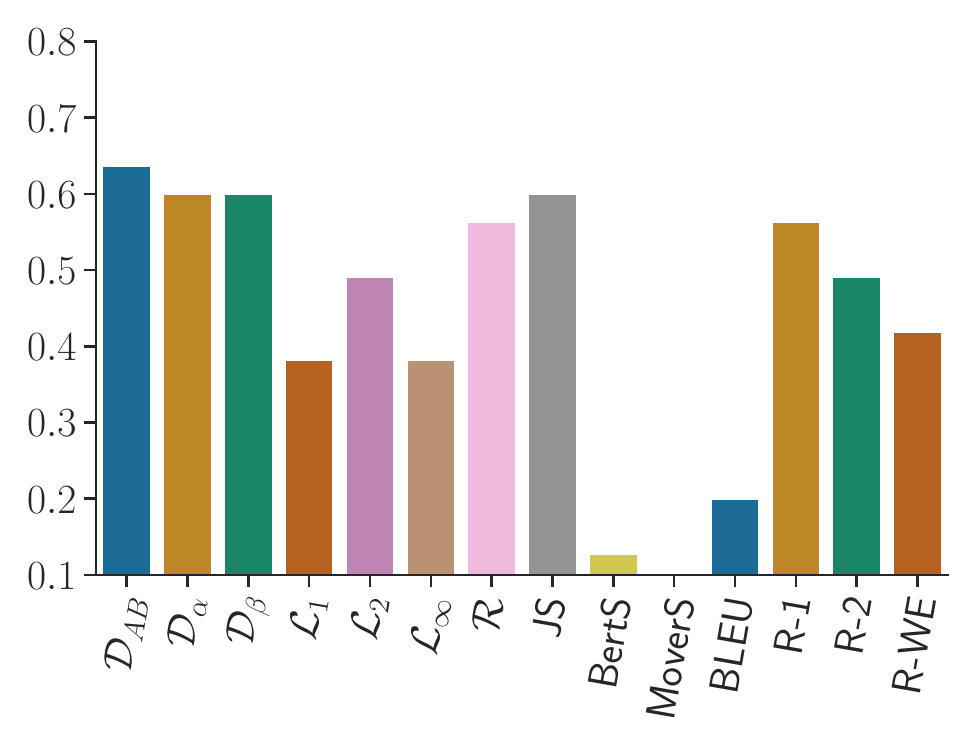}}\vspace{-.15cm}
\end{tabular}}
\caption{Results of the correlation between metrics and human judgement on the CNN dataset. % First, second and third row report correlations as measured by the Person ($r$), Spearman ($\rho$) and Kendall ($\tau$) coefficient respectively. %First, second and third, fourth columns report correlation coefficient at the text level (Text) where third and fourth columns report correlation at the system level (Sys). First and third column are dedicated to abstractive systems (Abs), second and fourth row report results for extractive systems. 
}\label{fig:cnn_results_all}
\end{figure*}
% appendix. 

\begin{figure*}\vspace{-0.5cm}
\centering
\subfloat[Score distribution Abstractive Summarization Systems]{\resizebox{\textwidth}{!}{\includegraphics{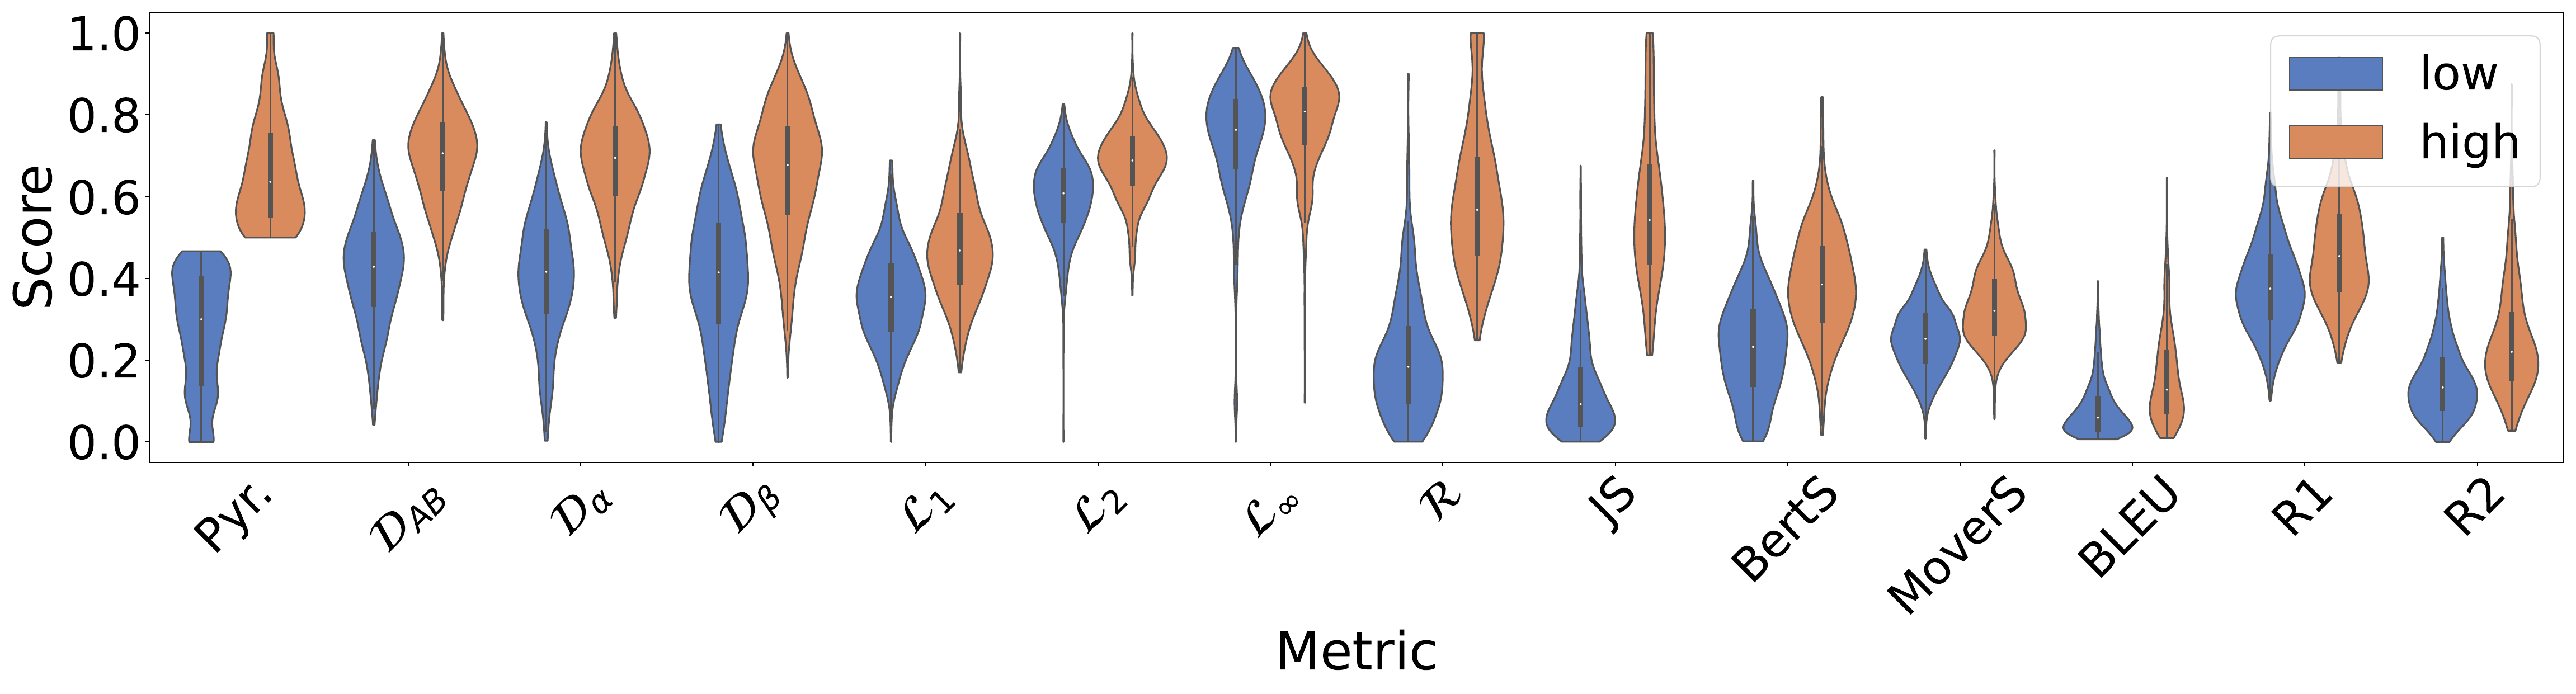}}}  \\
\subfloat[Score distribution Extractive Summarization Systems]{\resizebox{\textwidth}{!}{\includegraphics{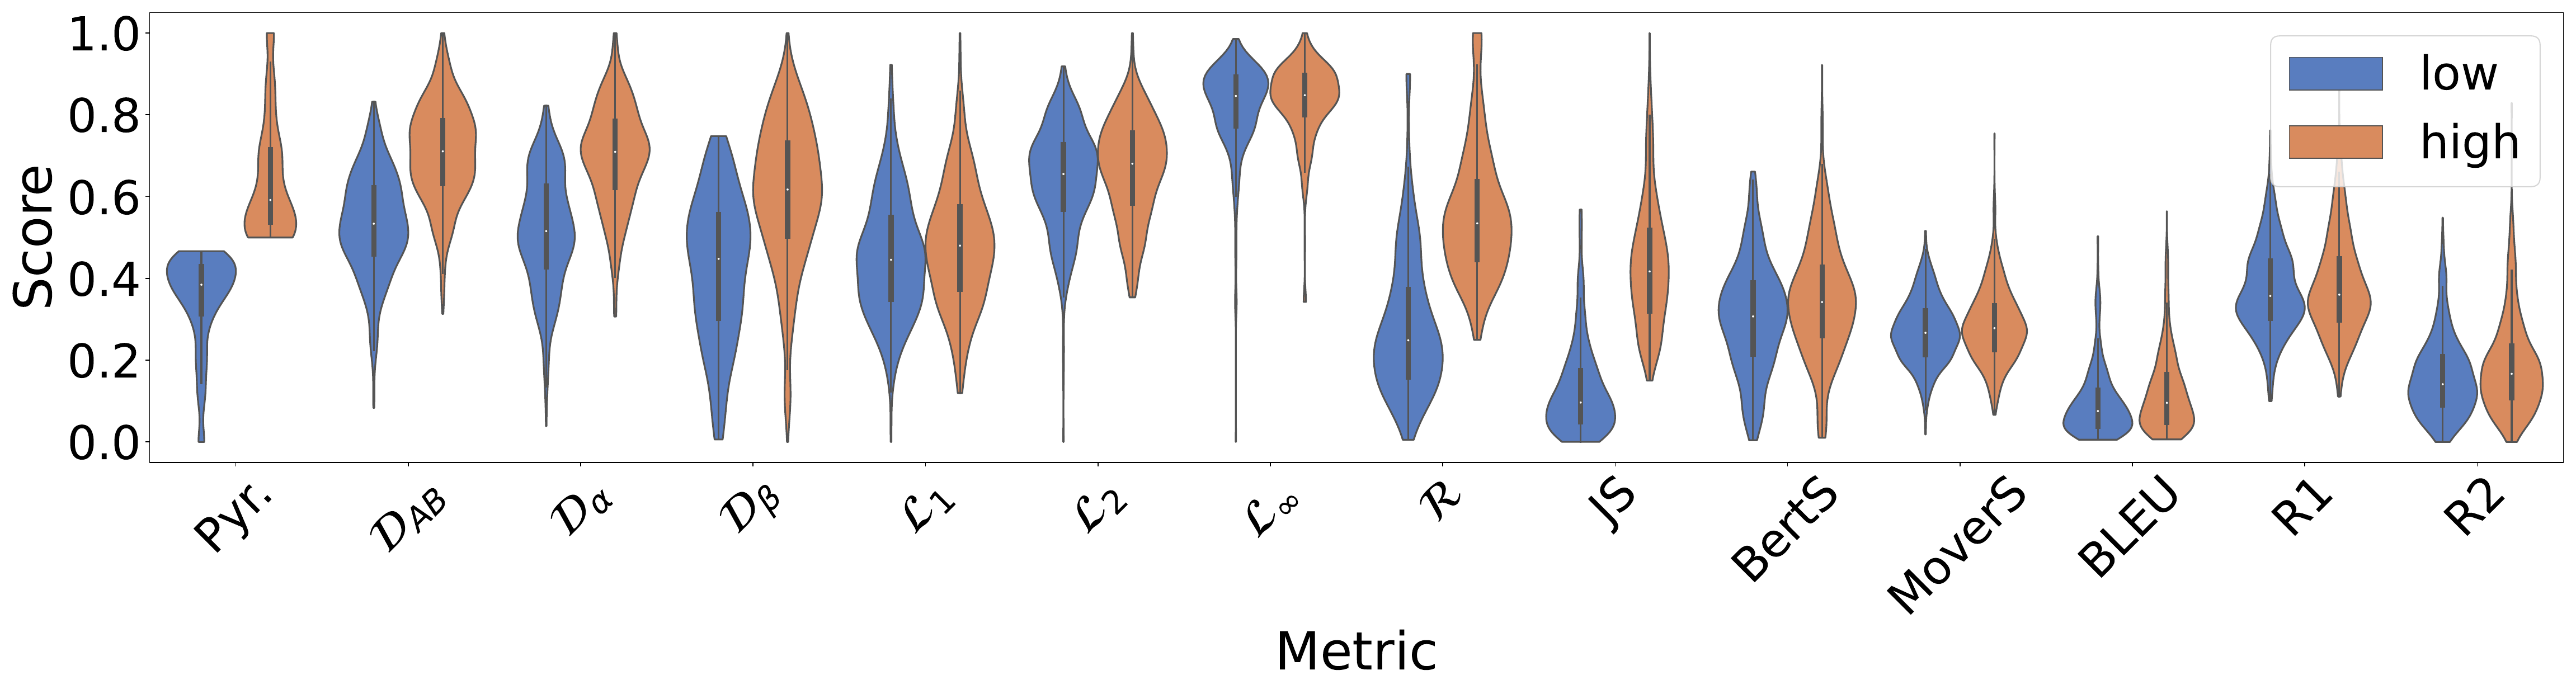}}}  \\
\caption{Score distribution considering a larger number of metrics than in \cref{fig:score_distrib_small}.}\label{fig:score_distribation}
\end{figure*}

\subsection{Parameters Choices}\label{ssec:all_results_on_cnn_additional}
For summarization (see \cref{fig:cnn_results_all}) we choose to work with the following parameters:
\begin{itemize}
    \item The temperature is set $1$.
        \item For $\mathcal{D}_\alpha$, we choose $\alpha = 0.75$ for extractive and  $\alpha = 3$ for abstractive.
        \item For $\mathcal{D}_\gamma$, we choose $\beta = 0.5$.
                \item For $\mathcal{D}_{AB}$, we choose $\beta = 0.25$  and $\alpha = 0.5$ for extractive and $\beta = 0.25$  and $\alpha = 3$ for abstractive.
\end{itemize}

For data2text generation (see \cref{ssec:complete_results_data2text}) we choose to work with the following parameters:
\begin{itemize}
    \item The temperature is set $1$.
    \item For $\mathcal{D}_\alpha$, we choose $\alpha = 0.75 $
        \item For $\mathcal{D}_\gamma$, we choose $\beta = 3 $
                \item For $\mathcal{D}_{AB}$, we choose $\beta = 0.25 ,\alpha=3$
\end{itemize}

\textbf{Takeaways} Although, parameters can be tuned to achieve better results. It is worth noting that the parameter-free Fisher-Rao distance (\textit{i.e.} $\mathcal{R}$) achieve good results when considered for \texttt{InfoLM}.

\section{Implementation details}\label{sec:algorithm_details}
\subsection{Algorithm details}
A complete algorithm for \texttt{InfoLM} is given in \cref{alg:infolm}.
\begin{algorithm}
  \caption{\texttt{InfoLM}
    \label{alg:infolm}}
  \begin{algorithmic}[1]
   \\\textsc{Input} Candidate text $\pmb{y}_i^s$ of length L, Reference text $\pmb{x_i}$ of length M, measure of information $\mathcal{I}$
\State $p_{\mathbf{\Omega} | \mathbf{T}}(\cdot |\pmb{y}_i^s), p_{\mathbf{\Omega} | \mathbf{T}}(\cdot |\pmb{x})= 0,0$
\For{\texttt{ $k \in [1,L]$}} \Comment{Compute $p_{\mathbf{\Omega} | \mathbf{T}}(\cdot |\pmb{y}_i^s)$}
                \State $p_{\mathbf{\Omega} | \mathbf{T}}(\cdot |\pmb{y_i^s}) = p_{\mathbf{\Omega} | \mathbf{T}}(\cdot |\pmb{y_i^s})  +  \gamma_k \times p_{\mathbf{\Omega} | \mathbf{T}}(\cdot |[\pmb{y}_i^s]^k) $
      \EndFor
      
\For{\texttt{ $j \in [1,M]$}} \Comment{Compute $p_{\mathbf{\Omega} | \mathbf{T}}(\cdot |\pmb{x_i})$}
                \State $p_{\mathbf{\Omega} | \mathbf{T}}(\cdot |\pmb{x_i}) = p_{\mathbf{\Omega} | \mathbf{T}}(\cdot |\pmb{x_i}) +  \bar{\gamma_k} \times p_{\mathbf{\Omega} | \mathbf{T}}(\cdot |[\pmb{x_i}]^j) $
      \EndFor
\\\textsc{Output} $\mathcal{I}\big[p_{\mathbf{\Omega} | \mathbf{T}}(\cdot |\pmb{y_i^s}),p_{\mathbf{\Omega} | \mathbf{T}}(\cdot|\pmb{x_i})\big]$
  \end{algorithmic}
\end{algorithm}
\subsection{Computational resources}
For all the experiments we use Tesla NVIDIA P100 to compute the BERT based metrics. Running time is less than an hour. For metrics based on string matching, we use a single CPU and the running time is less than an hour.
\subsection{Libraries}
For this project among the library we used we can cite: 
\begin{itemize}
    \item Transformers from \citet{hugging_face}.
    \item SummEval can be found here \url{https://github.com/Yale-LILY/SummEval} and has been proposed in \citet{fabbri2020summeval} for the dataset CNN.
    \item RealSumm  which can be found here \url{https://github.com/neulab/REALSumm} and has been proposed in \citet{bhandari2020re} for some metrics.
    \item Pytorch \cite{pytorch} for the GPU support.
    \item Implementation of \texttt{MOVERSCORE} can be found here \url{https://github.com/AIPHES/emnlp19-moverscore}.
    \item Implementation of \texttt{BERTSCORE} can be found here \url{https://github.com/Tiiiger/bert_score}.
        \item SacreBLEU for \texttt{BLEU} implementation \cite{sacrebleu}.
        \item The William test is taken from the author's code and is available at \url{https://github.com/ygraham/nlp-williams}
\end{itemize}
We thank the contributor for open-sourcing their libraries.
\subsection{Negative Results}
We tried to remove the stop words and do pre-processing technics. Little improvement when cleaning the candidate and golden reference text might be attributed to BERT.
